# Supplementary material for: Transformers versus the EM Algorithm in Multi-class Clustering
Source: arXiv:2502.06007 source file (2025-02-09)
Supplement: Supplementary file 1 [file sectappendix.tex]

\appendix

% {
% \setlength{\parskip}{-0em}
% \startcontents[sections]
% \printcontents[sections]{ }{1}{}
% }

% \stopcontents
% \startcontents[sections]
% \printcontents[sections]{ }{1}{}

\section{Additional Theoretical Background}

\begin{definition}[Sufficiently Smooth $d$-variate function]
    Denote $\msf B_{\infty}^d(R):=[-R,R]^d$ as the standard $\ell_\infty$ ball in $\bb R^d$.
    We say a function $g:\bb R^d\to\bb R$ is $(R,C_\ell)$ smooth if for $s=\lceil(d-1)/2\rceil+2$, $g$ is a $C^s$ function on $\msf B^d_\infty(\bb R)$ and
    \begin{align*}
        \sup_{\bfa z\in\msf B_{\infty}^d(R)}\Vert\nabla^dg(\bfa z)\Vert_{\infty}=\sup_{\bfa z\in\msf B^d_\infty(R)}\max_{j_1,\ldots,j_i\in[d]}\lef|\pta_{x_{j_1}\ldots x_{j_{i}}}g(\bfa x)\rig|\leq L_i
    \end{align*}
    for all $i\in\{0,1,\ldots,s\}$, with $\max_{0\leq i\leq s}L_iR^i\leq C_\ell$.
\end{definition}
\begin{definition}[Approximability by sum of Relus \citep{bai2024transformers}]\label{def6} A function $g:\bb R^k\to\bb R$ is $(\epsilon_{approx}, R,M,C)$-approximable by sum of Relus if there exists a function $f_{M,C}$ such that
\begin{align*}
    f_{M,C}(\bfa z)=\sum_{m=1}^Mc_m\sigma(\bfa a_m^\top[\bfa z;1])\text{ with }\sum_{m=1}^M|c_m|\leq C,\;\max_{m\in[M]}\Vert \bfa a_m\Vert_1\leq 1,\quad \bfa a_m\in\bb R^{k+1},\; c_m\in\bb R,
\end{align*}
such that $\sup_{\bfa z\in\msf B_\infty^k(R)}|g(\bfa z)-f_{M,C}(\bfa z)|\leq \epsilon_{approx}$.
\end{definition}

\section{Proofs}
\subsection{Proof of Proposition \ref{genbound}}
\begin{proof}
    The proof follows from \citep{wainwright2019high}, using the fact that for all $\bfa\theta\in \Theta(B_{\bfa\theta},B_M)$, we have 
    \begin{align*}
        \frac{1}{n}\sum_{j=1}^nL\lef(TF_{\wha\theta}(\bfa H_i),\bfa V_i\rig)\leq\frac{1}{n}\sum_{j=1}^n L\lef(TF_{\bfa\theta}(\bfa H_i),\bfa V_i\rig),
    \end{align*} 
    it is not hard to show that
    \begin{align*}
        \bb E\lef[L\lef(TF_{\wha\theta}(\bfa H),\bfa V\rig)\rig]\leq \inf_{\bfa\theta\in \Theta(B_{\bfa\theta},B_M)}\bb E\lef[L(TF_{\wha\theta}(\bfa H),\bfa V)\rig]+2\sup_{\bfa\theta\in \Theta(B_{\bfa\theta},B_M)}| X_{\bfa\theta}|,
    \end{align*}
    where $ X_{\bfa\theta}=\frac{1}{n}\sum_{j=1}^nL(TF_{\bfa\theta}(\bfa H_i),\bfa V_i)-\bb E[L(TF_{\bfa\theta}(\bfa H),\bfa V)]$ is the empirical process indexed by $\bfa\theta$.
    The tail bound for the empirical process requires us to verify a few regularity conditions \citep{gine2016mathematical} on the function $L$ and the set $\Theta$
    \begin{enumerate}
        \item The metric entropy of an operator norm ball $\log N(\delta, B_{\Vert\cdot\Vert_{op}}(r),\Vert\cdot\Vert_{op})\leq CLB_M D^2\log\lef(1+2(B_{\theta}+B_X+k)/\delta\rig)$.
        \item $L(TF_{\bfa\theta}(\bfa H),\bfa V)\leq C\sqrt k$.
        \item The Lipschitz condition of Transformers satisfies that for all $\bfa\theta_1,\bfa\theta_2\in\Theta(B_{\bfa\theta}, B_{M})$, we have $L(TF_{\bfa\theta_1}(\bfa H),\bfa V) - L(TF_{\bfa\theta_2}(\bfa H),\bfa V)\leq C L B_1^{L}\Vert\bfa\theta_1-\bfa\theta_2\Vert_{op}$ where $B_1=B_{\theta}^4B_X^3$.
    \end{enumerate}
    The first and second verifications follow immediately from J.2 in \citep{bai2024transformers}. The third verification is given upon noticing that as $L(\bfa x,\bfa y)=\Vert\bfa x-\bfa y\Vert_2$,
    \begin{align*}
        \sup_{\bfa\theta,\bfa H,\bfa V}L(TF_{\bfa\theta}(\bfa H),\bfa V)\leq C\sqrt k,\qquad \Vert\nabla_{\bfa x} L\Vert\leq C.
    \end{align*}
    Further note that $\Vert\tda W_0\Vert_2\asymp\Vert\tda W_1\Vert_2\asymp 1$.
    Given the above result, and corollary J.1 in \citep{bai2024transformers}, we can show that
    \begin{align*}
        L(TF_{\bfa\theta_1}(\bfa H),\bfa V)-L(TF_{\bfa\theta_2}(\bfa H),\bfa V)\leq C L B_1^{L}\Vert\bfa\theta_1-\bfa\theta_2\Vert_{op},
    \end{align*}
    where $B_1 = B^4_{\theta}B^3_{X}$.
    Therefore, using the uniform concentration bound given by proposition A.4 we can show that with probability at least $1-\xi$, we have
    \begin{align*}
        \sup_{\bfa\theta\in\Theta(B_{\bfa\theta},B_M)} |X_{\theta}|\leq C\sqrt k\sqrt{\frac{LB_MD^2\log(B_{\theta}+B_X+k)+\log(1/\delta)}{n}}.
    \end{align*}
    Therefore, replacing $D$ with $Ckd$ we complete the proof.
\end{proof}

\subsection{Proof of Theorem \ref{thm3.1}}
\begin{proof}
    Our proof can be dissected into the following steps: 1. We construct a Transformer with fixed parameters that performs
    (1) The computation of the symmetrized covariate matrix; (2) The approximation of the power method; (3) The removal of the principal eigenvectors; (4) Adjust the dimension of the output through multiplying the two matrices $\tda W_0$ and $\tda W_1$ on the left and right.
    \begin{center}
        \textbf{1. The Covariate Matrix.}
    \end{center}
    To compute the covariate matrix $\bfa X\bfa X^\top$, we construct $\bfa H=\begin{bmatrix}
        \bfa X_1,\ldots,\bfa X_N\\
        \tda p_{1,1},\ldots,\tda p_{1,N}\\
        \tda p_{2,1},\ldots,\tda p_{2,N}\\
        \vdots\\
        \tda p_{\ell,1},\ldots,\tda p_{\ell,N}
    \end{bmatrix}=\begin{bmatrix}
        \bfa X\\
        \bfa P
    \end{bmatrix}$
    we let $m=2$ and
    \begin{align}
     & \bfa V_1^{cov}=I_D=-\bfa V_2^{cov},\quad \bfa Q_1^{cov,\top}\bfa K_1^{cov}=-\bfa Q_2^\top\bfa K_2=\begin{bmatrix}
         \bfa 0_{N+1\times d}, I_d,\bfa 0\\
         \bfa 0,\bfa 0,\bfa 0
     \end{bmatrix}\in\bb R^{D\times D},\nnb\\
     &\tda p_{1,\ell,j}=\bfa 0,\qquad\tda p_{2,\ell,j}=\begin{cases}
         \mbbm 1_{\ell=j}\quad&\text{ when }\ell\leq d\\
         0&\text{ when }\ell>d
     \end{cases}.
    \end{align}
    Under the above construction, we obtain that
    \begin{align*}
        &\bfa Q_1^\top\bfa K_1\bfa H=\begin{bmatrix}
            I_{d}&\bfa 0\\
            \bfa 0&\bfa 0
        \end{bmatrix}\in\bb R^{D\times N},\quad\bfa Q_2^\top\bfa K_2\bfa H=\begin{bmatrix}
            -I_{d}&\bfa 0\\
            \bfa 0&\bfa 0
        \end{bmatrix}\in\bb R^{D\times N},\\
        &\sigma(\bfa H^\top\bfa Q_1^\top\bfa K_1\bfa H)+\sigma(\bfa H^\top\bfa Q_2^\top\bfa K_2\bfa H)=\begin{bmatrix}
            \bfa X^\top,\bfa 0
        \end{bmatrix}\in\bb R^{N\times N}.
    \end{align*}
   We further obtain that
    \begin{align*}
        \frac{1}{N}\sum_{m=1}^M(\bfa V_m\bfa H)\times \sigma\lef((\bfa Q_m\bfa H)^\top(\bfa K_m\bfa H)\rig)=\begin{bmatrix}
        \bfa 0&\bfa 0\\
            \bfa X\bfa X^\top\in\bb R^{d\times d}&\bfa 0\\
            \bfa 0&\bfa 0
        \end{bmatrix}\in\bb R^{D\times D}.
    \end{align*}
    Therefore, the output is given by  $\tda H^{cov}=\begin{bmatrix}
            \bfa X\\
            \bfa X\bfa X^\top,\bfa 0\\
            \tda p_{2,1},\ldots,\tda p_{2,N}\\
            \tda p_{\ell,1},\ldots,\tda p_{\ell,N}
        \end{bmatrix}$. 
    \begin{center}
        \textbf{2. The Power Iteration.}
    \end{center}
    Then we consider constructing a single attention layer that approximates the power iteration. This step involves two important operations: (1) Obtaining the vector given by $\bfa X\bfa X^\top\bfa v$. (2) Approximation of the value of the inverse norm given by $1/\Vert \bfa X\bfa X^\top\bfa v\Vert_2$. We show that one can use the multi-head Relu Transformer to achieve both goals simultaneously, whose parameters are given by 
    \begin{align*}
        \bfa V_{1}^{pow,1}&=-\bfa V_{2}^{pow,1}=\begin{bmatrix}
            \bfa 0_{(3d+1)\times (2d+1)}&\bfa 0&\bfa 0\\
            \bfa 0_{(d)\times(2d+1)}&I_d&\bfa 0\\
            \bfa 0&\bfa 0&\bfa 0
        \end{bmatrix},\\
        \bfa Q_1^{pow,1}&=-\bfa Q_1^{pow,1}=\begin{bmatrix}
           \bfa 0_{(d+1)\times (d+1)}& \bfa 0&\bfa 0\\
            \bfa 0_{d\times (d+1)}&I_d&\bfa 0\\
            \bfa 0&\bfa 0&\bfa 0
        \end{bmatrix},\\
        \bfa K_1^{pow,1}&=\bfa K_2^{pow,1}=\begin{bmatrix}
            \bfa 0_{(3d+1)\times(3d+1)}&\bfa 0&\bfa 0\\
            \bfa 0_{d\times(3d+1)}&I_d&\bfa 0\\
            \bfa 0&\bfa 0&\bfa 0
        \end{bmatrix},\qquad\tda p_{4,j} = \bfa 0\text{ for all }j\in[N].
    \end{align*}
    Given the above formulation, we can show that 
    \begin{align*}
       &\bfa Q_2^{pow,1}\tda H^{cov}=-\bfa Q_1^{pow,1}\tda H^{cov} = \begin{bmatrix}
        \bfa 0_{(2d+1)\times N}\\
            \bfa X\bfa X^\top,\bfa 0\\
            \bfa 0
        \end{bmatrix},\\
        &\bfa K_2^{pow,1}\tda H^{cov}=\bfa K_1^{pow,1}\tda H^{cov}=\begin{bmatrix}
            \bfa 0_{2d+1}\\
            \tda p_{3,1},\bfa 0\\
            \bfa 0
        \end{bmatrix},
    \end{align*}
    which implies that 
    \begin{align*}
    \sum_{m\in\{1,2\}}\sigma((\bfa Q_m^{pow, 1}\tda H^{cov})^\top\bfa K_m^{pow,1}\tda H^{cov})=\begin{bmatrix}
           \bfa 0& \bfa 0_{d\times(2d+1)}&\\
            \bfa X\bfa X^\top\tda p_{3,1}&\bfa 0_{d\times(N-1)}\\
            \bfa 0&\bfa 0&
        \end{bmatrix}.
    \end{align*}
    Then we can show that 
    \begin{align*}
        \tda H^{pow,1}-\tda H^{cov}&=\sum_{m\in\{1,2\}}\bfa V_m^{pow,1}\tda H^{cov}\times\sigma((\bfa Q_m^{pow,1}\tda H^{cov})^\top\bfa K_m^{pow,1}\tda H^{cov})\\
        &=\begin{bmatrix}
            \bfa 0_{3d+1}\\
            \bfa X\bfa X^\top\tda p_{3,1},\bfa 0_{d\times(N-1)}\\
            \bfa 0
        \end{bmatrix}.
    \end{align*}
    Therefore, we conclude that the output of the first power iteration layer is given by
    \begin{align*}
        \tda H^{pow,1}=\begin{bmatrix}
            \bfa X\\
            \tda y^\top\\
            \bfa X\bfa X^\top,\bfa 0\\
            \tda p_{2,1},\ldots,\tda p_{2,N}\\
            \tda p_{3,1},\ldots,\tda p_{3,N}\\
            \bfa X\bfa X^\top\tda p_{3,1},\bfa 0\\
            \tda p_{5,1},\ldots,\tda p_{5,N}\\
            \vdots\\
            \tda p_{\ell,1},\ldots,\tda p_{\ell,N}
        \end{bmatrix}.
    \end{align*}
    % Then we consider integrating the normalizing constants into $\bfa H$ and remove unnecessary $\tda p_{}$.
    % We further let $\tda p_{3,\ell}$ to be i.i.d. sampled from $\bb S^{d-1}$ and one uses lemma \ref{reluapprox} to obtain that there exists $\{\bfa a_m\}_{m\in[M]}$ with
    % \begin{align*}
    %     \frac{1}{N}\sum_{m=1}^M(\bfa V_m\bfa H)\times\sigma\lef((\bfa Q_m\bfa H)^\top(\bfa K_m\bfa H)\rig)=\begin{bmatrix}
    %         \bfa 0_{(4d+1)\times N}\\
    %         \frac{\bfa X\bfa X^\top\tda p_{1,1}}{\Vert\bfa X\bfa X^\top\tda p_{1,1}\Vert_2},\ldots,\bfa 0\\
    %         \bfa 0
    %     \end{bmatrix}.
    % \end{align*}
    Then, using lemma \ref{reluapprox}, we design an extra attention layer that performs the normalizing procedure, with the following parameters for all $m\in[M]$,
    \begin{align*}
        &\bfa V_{m}^{pow,2}=\begin{bmatrix}
            \bfa 0_{d\times (4d+1)}&c_m\bfa I_d&\bfa 0\\
            \bfa 0&\bfa 0&\bfa 0
        \end{bmatrix},\qquad\bfa Q_{m}^{pow,2}=\begin{bmatrix}
            \bfa 0_{d\times(2d+1)}&\bfa I_{d}&\bfa 0\\
            \bfa 0&\bfa 0&\bfa 0
        \end{bmatrix},\\
        &\bfa K_m^{pow,2}=\begin{bmatrix}
            \bfa 0_{1\times (3d+1)}&\bfa a_m^\top&\bfa 0\\
            \vdots\\
            \bfa 0_{1\times(3d+1)}&\bfa a_m^\top&\bfa 0\\
            \bfa 0_{(D-d)\times(3d+1)}&\bfa 0&\bfa 0
        \end{bmatrix}.
    \end{align*}
    Under the above construction, we obtain that
    \begin{align*}
        (\bfa Q_m^{pow,2}\tda H^{pow,1})^\top =\begin{bmatrix}
            I_{d\times d}&\bfa 0\\
            \bfa 0&\bfa 0
        \end{bmatrix},\qquad \bfa K_m^{pow,2}\tda H^{pow,1} = \begin{bmatrix}
            \bfa a_m^\top\bfa X\bfa X^\top\tda p_{3,1}&\bfa 0\\
            \vdots\\
            \bfa a_m^\top\bfa X\bfa X^\top\tda p_{3,1}&\bfa 0\\
            \bfa 0_{(D-d)\times 1}&\bfa 0
        \end{bmatrix}.
    \end{align*}
    Then, given $\bfa V_m^{pow,2}$ we can show that under the condition given by lemma \ref{reluapprox}, we have
    \begin{align*}
        \bigg\Vert&\sum_{m=1}^M\bfa V_m^{pow,2}\tda H^{pow,1}\sigma\lef((\bfa Q_m^{pow,2}\tda H^{pow,1})^\top(\bfa K_m^{pow,2}\tda H^{pow,1})\rig)-\begin{bmatrix}
        \bfa 0_{4d+1}\\
            \frac{\bfa X\bfa X^\top\tda p_{3,1}}{\Vert\bfa X\bfa X^\top\tda p_{3,1}\Vert_2}-\bfa X\bfa X^\top\tda p_{3,1},\bfa 0\\
            \bfa 0
        \end{bmatrix}\bigg\Vert_{\infty}\\
        &<\epsilon,
    \end{align*}
    Moreover, we can further achieve that
    \sm{\begin{align*}
        \Bigg\Vert\sum_{m=1}^M\bfa V_m^{pow,2j}\tda H^{pow,1}\sigma\lef((\bfa Q_m^{pow,2}\tda H^{pow,1})^\top (\bfa K_m^{pow,2}\tda H^{pow,1})\rig)&-\begin{bmatrix}
            \bfa 0_{4d+1}\\
            \frac{\bfa X\bfa X^\top\tda p_{3,1}}{\Vert\bfa X\bfa X^\top\tda p_{3,1}\Vert_2}-\bfa X\bfa X^\top\tda p_{3,1},\bfa 0\\
            \bfa 0
        \end{bmatrix}\Bigg\Vert_2\\
        &<\epsilon\Vert\bfa X\bfa X^\top\tda p_{3,1}\Vert_2.
    \end{align*}}
    Hence, using the fact that $\tda H^{pow,2}=\tda H^{pow,1}+\sum_{i=1}^m\bfa V_m^{pow,2}\tda H^{pow,1}\sigma\lef((\bfa Q_m^{pow,2}\tda H^{pow,1})^\top(\bfa K_m^{pow,2}\tda H^{pow,1})\rig)$, we obtain that
    \begin{align*}
        \Bigg\Vert\tda H^{pow,2}-\begin{bmatrix}
            \bfa X\\
            \tda y\\
            \bfa X\bfa X^\top,\bfa 0\\
            \tda p_{2,1},\ldots,\tda p_{2,N}\\
            \tda p_{3,1},\ldots,\tda p_{3,N}\\
            \frac{\bfa X\bfa X^\top\tda p_{3,1}}{\Vert\bfa X\bfa X^\top\tda p_{3,1}\Vert_2},\ldots\bfa 0\\
            \vdots
        \end{bmatrix}\Bigg\Vert_{2}<\epsilon\Vert\bfa X\bfa X^\top\tda p_{3,1}\Vert_2.
    \end{align*}
    Then we construct another attention layer, which performs similar calculations as that of $pow,1$ but switch the rows of $\tda p_{3,1}$ with that of $\frac{\bfa X\bfa X^\top\tda p_{3,1}}{\Vert\bfa X\bfa X^\top\tda p_{3,1}\Vert_2}$. Our construction for the third layer is given by
    \begin{align*}
        \bfa V_{1}^{pow,3}&=-\bfa V_{2}^{pow,3}=\begin{bmatrix}
            \bfa 0_{(3d+1)\times (2d+1)}&\bfa 0&\bfa 0\\
            \bfa 0_{d\times(2d+1)}&I_d&\bfa 0\\
            \bfa 0&\bfa 0&\bfa 0
        \end{bmatrix},\\
        \bfa Q_1^{pow,3}&=-\bfa Q_2^{pow,3}=\begin{bmatrix}
           \bfa 0_{(3d+1)\times (d+1)}&\bfa 0& \bfa 0\\
            \bfa 0_{d\times (d+1)}&I_d&\bfa 0\\
            \bfa 0&\bfa 0&\bfa 0
        \end{bmatrix},\\
        \bfa K_1^{pow,3}&=\bfa K_2^{pow,3}=\begin{bmatrix}
            \bfa 0_{(4d+1)\times(4d+1)}&\bfa 0&\bfa 0\\
            \bfa 0_{d\times(4d+1)}&I_d&\bfa 0\\
            \bfa 0&\bfa 0&\bfa 0
        \end{bmatrix},\qquad\tda p_{4,j} = \bfa 0\text{ for all }j\in[N].
    \end{align*}
    Given the above construction, we can show that
    \begin{align*}
       &\bfa Q_2^{pow,3}\tda H^{pow,2}=-\bfa Q_1^{pow,3}\tda H^{pow,2}=\begin{bmatrix}
           &\bfa 0_{(3d+1)\times N}&\\
           \bfa 0_{}&\bfa X\bfa X^\top &\bfa 0\\
           &\bfa 0&
       \end{bmatrix},\quad \bfa K_2^{pow,3}\tda H^{pow,2}=\bfa K_1^{pow,3}\tda H^{pow,2},\\
       &\Bigg\Vert\bfa K_2^{pow,3}\tda H^{pow,2}-\begin{bmatrix}
            \bfa 0_{(3d+1)\times N}\\
            \frac{\bfa X\bfa X^\top\tda p_{3,1}}{\Vert\bfa X\bfa X^\top\tda p_{3,1}\Vert_2},\bfa 0\\
            \bfa 0
        \end{bmatrix}\Bigg\Vert_{2}\leq\epsilon\Vert\bfa X\bfa X^\top\tda p_{3,1}\Vert_2.
    \end{align*}
    Then, using the fact that given $\bfa x_1,\bfa x_2$ with $\Vert\bfa x_1-\bfa x_2\Vert_2\leq\delta_0$, we have
$        \Vert\bfa X\bfa X^\top(\bfa x_1-\bfa x_2)\Vert_2\leq \Vert\bfa X\bfa X^\top\Vert_2\delta_0 $. 
    Hence, by collecting the above pieces, we have
    \begin{align*}
      \Bigg\Vert\sum_{m=1}^2\bfa V_m^{pow,3}\tda H^{pow,2}\sigma\lef((\bfa Q_2^{pow,3}\tda H^{pow,2})^{\top}\bfa K_2^{pow,3}\tda H^{pow,2}\rig)&-\begin{bmatrix}
          \bfa 0_{(3d+1)\times N}\\
          \frac{(\bfa X\bfa X^\top)^2\tda p_{3,1}}{\Vert\bfa X\bfa X^\top\tda p_{3,1}\Vert_2}-\frac{\bfa X\bfa X^\top\tda p_{3,1}}{\Vert\bfa X\bfa X^\top\tda p_{3,1}\Vert_2},\bfa 0\\
          \bfa 0
      \end{bmatrix}\Bigg\Vert_{2}\\
      &\leq\epsilon\Vert\bfa X\bfa X^\top\Vert_2\lef\Vert\bfa X\bfa X^\top\tda p_{3,1}\rig\Vert_2.
    \end{align*}
    Henceforth, one can further show that
$      \Bigg\Vert \tda H^{pow,3}- \begin{bmatrix}
            \bfa X\\
            \tda y\\
            \bfa X\bfa X^\top,\bfa 0\\
            \tda p_{2,1},\ldots,\tda p_{2,N}\\
            \tda p_{3,1},\ldots,\tda p_{3,N}\\
            \frac{(\bfa X\bfa X^\top)^2\tda p_{3,1}}{\Vert\bfa X\bfa X^\top\tda p_{3,1}\Vert_2},\bfa 0\\
            \tda p_{5,1},\ldots,\tda p_{5,N}\\
            \vdots\\
            \tda p_{\ell,1},\ldots,\tda p_{\ell,N}
        \end{bmatrix}\Bigg\Vert_{2}\leq\epsilon \Vert\bfa X\bfa X^\top\Vert_2\Vert\bfa X\bfa X^\top\tda p_{3,1}\Vert_2$.
    Consider we are doing in total of $\tau$ power iterations, we can set for all $\tau\in\bb N^*$,
    \begin{align*}
        &\bfa V_m^{pow,2\tau+1}=\bfa V_m^{pow,3},\quad \bfa Q_m^{pow,2\tau+1}=\bfa Q_m^{pow,3},\quad\bfa K_m^{pow,2\tau+1}=\bfa K_m^{pow,3},\\
        &\bfa V_m^{pow,2\tau+2}=\bfa V_m^{pow,4},\quad\bfa Q_m^{pow,2\tau+2}=\bfa Q_m^{pow,4},\quad\bfa K_m^{pow,2\tau+2}=\bfa K_m^{pow,4}.
    \end{align*}
    Therefore, taking another layer of normalization, we can show that
    \begin{align*}
        \Bigg\Vert \tda H^{pow,3}- \begin{bmatrix}
            \bfa X\\
            \tda y\\
            \bfa X\bfa X^\top,\bfa 0\\
            \tda p_{2,1},\ldots,\tda p_{2,N}\\
            \tda p_{3,1},\ldots,\tda p_{3,N}\\
            \frac{(\bfa X\bfa X^\top)^2\tda p_{3,1}}{\Vert\bfa X\bfa X^\top\tda p_{3,1}\Vert_2^2},\bfa 0\\
            \tda p_{5,1},\ldots,\tda p_{5,N}\\
            \vdots\\
            \tda p_{\ell,1},\ldots,\tda p_{\ell,N}
        \end{bmatrix}\Bigg\Vert_{2}\leq2\epsilon \Vert\bfa X\bfa X^\top\Vert_2.
    \end{align*}
    Then, using the sublinearity of errors, we can show that for $\tau\in\bb N$,
    \begin{align*}
              \Bigg\Vert \tda H^{pow,2\tau+2}- \begin{bmatrix}
            \bfa X\\
            \tda y\\
            \bfa X\bfa X^\top,\bfa 0\\
            \tda p_{2,1},\ldots,\tda p_{2,N}\\
            \tda p_{3,1},\ldots,\tda p_{3,N}\\
            \tda p_{3,1}^{(\tau)},\bfa 0\\
            \tda p_{5,1},\ldots,\tda p_{5,N}\\
            \vdots\\
            \tda p_{\ell,1},\ldots,\tda p_{\ell,N}
        \end{bmatrix}\Bigg\Vert_{\infty}\leq \tau\epsilon\Vert\bfa X\bfa X^\top\Vert_2,\quad\tda p^{(\tau)}_{3,1}=\frac{\bfa X\bfa X^\top\tda p_{3,1}^{(\tau-1)}}{\lef\Vert\bfa X\bfa X^\top\tda p_{3,1}^{(\tau-1)}\rig\Vert_2},\quad\tda p_{3,1}^{(0)}=\tda p_{3,1}.
    \end{align*}
    If we denote $\bfa v_i$ as the eigenvector corresponds to the $i$ th largest eigenvalue of $\bfa X\bfa X^\top$. Let the eigenvalues of $\bfa X\bfa X^\top$ be denoted by $\lambda_1>\lambda_2>\cdots>\lambda_n$. Given $|\tda p_{3,1}^\top\bfa v_1|>\delta$ and $|\sqrt{\lambda_1}-\sqrt{\lambda_2}|=\Omega(1)$. Theorem 3.11 in \citep{blum2020foundations} page 53 shows that given $k=\frac{\log(1/\epsilon_0\delta)}{2\epsilon_0}$ and $\Vert\tda p_{3,1}^{(\tau)}\Vert_2 = \Vert\bfa v_1\Vert_2=1$, one immediately obtains that
    \begin{align*}  
    \tda p_{3,1}^{(\tau),\top}\bfa v_1\geq 1- \epsilon_0,\qquad\Vert\tda p_{3,1}^{(\tau)}-\bfa v_1\Vert_2 = \sqrt{2-2\bfa v_1^\top\tda p_{3,1}^{(\tau)}}=\sqrt{2\epsilon_0}.
    \end{align*}
    We also consider the approximation of the maximum eigenvalue. Note that using $\Vert\bfa v_1\Vert_2=1$, we have 
    \begin{align*}
       \Vert\bfa X\bfa X^\top\Vert_2&=\Vert\bfa X\bfa X^\top\bfa v_1\Vert_2=\lef\Vert\bfa X\bfa X^\top\tda p_{3,1}^{(\tau)}+\bfa X\bfa X^\top(\bfa v_1-\tda p_{3,1}^{(\tau)})\rig\Vert_2\\
       &\leq\Vert\bfa X\bfa X^\top\tda p_{3,1}^{(\tau)}\Vert_2+\Vert\bfa X\bfa X^\top(\bfa v_1-\tda p_{3,1}^{(\tau)})\Vert_2\\
       &\leq\Vert\bfa X\bfa X^\top\tda p_{3,1}^{(\tau)}\Vert_2+\Vert\bfa X\bfa X^\top\Vert_2\Vert\bfa v_1-\tda p_{3,1}^{(\tau)}\Vert_2.
   \end{align*}
   Similarly we can also derive that $\Vert\bfa X\bfa X^\top\Vert_2\geq \Vert\bfa X\bfa X^\top\tda p_{3,1}^{(\tau)}\Vert_2-\Vert\bfa X\bfa X^\top\Vert_2\Vert\bfa v_1-\tda p_{3,1}\Vert_2$. Then we show that
   \begin{align*}
       \Big|\Vert\bfa X\bfa X^\top\Vert_2-\Vert\bfa X\bfa X^\top\tda p_{3,1}^{(\tau)}\Vert_2\Big|\leq\Vert\bfa X\bfa X^\top\Vert_2\Vert\bfa v_1-\tda p_{3,1}^{(\tau)}\Vert_2\leq\sqrt{2\epsilon_0}\Vert\bfa X\bfa X^\top\Vert_2.
   \end{align*}
    \begin{center}
        \textbf{3. The Removal of Principal Eigenvectors.}
    \end{center}
    After $\tau$ iterates on the power method, we need to remove the principal term from the matrix $\bfa X\bfa X^\top$, achieved through two important steps: (1) The computation of the estimated eigenvalue $\Vert\bfa X\bfa X^\top\tda p_{3,1}\Vert_2$. (2) The construction of the low rank update $\tda p_{3,1}\tda p_{3,1}^\top$. For step (1), we consider the following construction:
    \begin{align*}
        &\bfa V_1^{rpe,1}=-\bfa V_2^{rpe,1}=\begin{bmatrix}
            \bfa 0_{(3d+1)\times(2d+1)}&\bfa 0&\bfa 0\\
            \bfa 0_{d\times(2d+1)}&I_d&\bfa 0\\
            \bfa 0&\bfa 0&\bfa 0
        \end{bmatrix},\quad\bfa Q_1^{rpe,1} =-\bfa Q_2^{rpe,1}= \begin{bmatrix}
            \bfa 0_{(d+1)\times(d+1)}&\bfa 0&\bfa 0\\
            \bfa 0_{d\times(d+1)}& I_d&\bfa 0\\
            \bfa 0&\bfa 0&\bfa 0
        \end{bmatrix},\\
        &\bfa K_1^{rpe,1}=\bfa K_2^{rpe,1} = \begin{bmatrix}
            \bfa 0_{(4d+1)\times(4d+1)}&\bfa 0&\bfa 0\\
            \bfa 0_{d\times(4d+1)}& I_d&\bfa 0\\
            \bfa 0&\bfa 0&\bfa 0
        \end{bmatrix}.
    \end{align*}
    Note that the above construction is similar to the first layer of the power method. Under this construction, we can show that
    \begin{align}\label{diffhrpe1}
        &\tda H^{rpe,1}=\tda H^{pow,2\tau+2}+\sum_{m\in\{1,2\}}\bfa V_m^{rpe,1}\sigma((\bfa Q_m^{rpe,1}\tda H^{pow,2\tau+2})^\top(\bfa K_m^{rpe,1}\tda H^{pow,2\tau+2})),\nnb\\
        &\Bigg\Vert\tda H^{rpe,1}-\ub{\begin{bmatrix}
            \bfa X\\
            \tda y\\
            \bfa X\bfa X^\top,\bfa 0\\
            \tda p_{2,1},\ldots,\tda p_{2,N}\\
            \tda p_{3,1},\ldots,\tda p_{3,N}\\
            \tda p_{3,1}^{(\tau)},\bfa 0\\
            \bfa X\bfa X^\top\tda p_{3,N}^{(\tau)},\bfa 0\\
            \tda p_{6,1},\ldots,\tda p_{6,N}\\
            \vdots\\
            \tda p_{\ell,1},\ldots,\tda p_{\ell,N}
        \end{bmatrix}}_{=:\bfa H^{rpe,1}}\Bigg\Vert_2\leq C\tau\epsilon\Vert\bfa X\bfa X^\top\Vert_2^2,\qquad\tda p_{5,i}=\bfa 0,\quad\forall i\in[N].
    \end{align}
    Then, we construct the next layer, using the notations in lemma \ref{reluapprox}, for $M\geq \Vert\bfa X\bfa X^\top\Vert_2^d\frac{C(d)}{\epsilon^2}$ for all $m\in[M]$ we have 
    \begin{align*}
       &\bfa V_m^{rpe,2}=\begin{bmatrix}
            \bfa 0_{d\times(4d+1)}&d_m\bfa I_d&\bfa 0\\
            \bfa 0&\bfa 0&\bfa 0
       \end{bmatrix},\qquad \bfa Q_m^{rpe,2} =\begin{bmatrix}
           \bfa 0_{d\times(2d+1)}&\bfa I_d&\bfa 0\\
           \bfa 0&\bfa 0&\bfa 0
       \end{bmatrix},\\
       &\bfa K_m^{rpe,2} =\begin{bmatrix}
           \bfa 0_{1\times(5d+1)}&\bfa b_m^\top&\bfa 0\\
           \vdots&&\\
           \bfa 0_{1\times(5d+1)}&\bfa b_m^\top&\bfa 0 \\
           \bfa 0_{(D-d)\times(5d+1)}&\bfa 0&\bfa 0
       \end{bmatrix}.
    \end{align*}
    Given the above construction, we subsequently show that
    \begin{align*}
       (\bfa Q_m^{rpe,2}\tda H^{rpe,1})^\top=\begin{bmatrix}
           I_{d\times d}&\bfa 0\\
           \bfa 0&\bfa 0
       \end{bmatrix},\qquad \bfa K_m^{rpe,2}\tda H^{rpe,1} = \begin{bmatrix}
            \bfa b_m^\top\bfa X\bfa X^\top\tda p_{3,1}^{(\tau)}&\bfa 0\\
            \vdots &\vdots\\
            \bfa b_m^\top\bfa X\bfa X^\top\tda p_{3,1}^{(\tau)}&\bfa 0\\
            \bfa 0_{(D-d)\times 1}&\bfa 0
        \end{bmatrix}.
    \end{align*}
    Hence, given the construction of $\bfa V_m^{rpe,2}$, we can show that $
        \tda H^{rpe,2} $ satisfies
        \begin{align*}
           \tda H^{rpe,2} &= \tda H^{rpe,1}+\sum_{m\in[M]}\bfa V_m^{rpe,2}\tda H^{rpe,1}\times\sigma\lef((\bfa K^{rpe,2}_m\tda H^{rpe,1})^\top(\bfa Q_m^{rpe}\tda H^{rpe,1})\rig)\\
           &=\ub{\bfa H^{rpe,1}+\sum_{m\in[M]}\bfa V_m^{rpe,2}\bfa H^{rpe,1}\times\sigma\lef((\bfa K_m^{rpe,2}\bfa H^{rpe,1})^\top(\bfa Q_m^{rpe,2}\bfa H^{rpe,1})\rig)}_{=:\wha H^{rpe,1}}\\
           &+\lef(\tda H^{rpe,1}-\bfa H^{rpe,1}\rig)+\sum_{m\in[M]}\bfa V_m^{rpe,2}\tda H^{rpe,1}\times\sigma\lef((\bfa K_m^{rpe,2}\tda H^{rpe,1})^\top\bfa Q_m^{rpe,2}\tda H^{rpe,1}\rig)\\
           &-\sum_{m\in[M]}\bfa V_m^{rpe,2}\tda H^{rpe,1}\times\sigma\lef((\bfa K_m^{rpe,2}\tda H^{rpe,1})^\top\bfa Q_m^{rpe,2}\tda H^{rpe,1}\rig).
        \end{align*}
    We note that by lemma \ref{reluapprox} we can show that
    \begin{align*}
        \Bigg\Vert\wha H^{rpe,1}-\begin{bmatrix}
            \bfa X\\
            \tda y\\
            \bfa X\bfa X^\top,\bfa 0\\
            \tda p_{2,1}\ldots,\tda p_{2,N}\\
            \tda p_{3,1}\ldots,\tda p_{3,N}\\
            \tda p_{3,1}^{(\tau)},\bfa 0\\
            \Vert\bfa X\bfa X^\top\tda p_{3,N}^{(\tau)}\Vert_2^{\frac{1}{2}}\tda p_{3,1}^{(\tau)},\bfa 0\\
            \vdots\\
            \tda p_{\ell,1},\ldots\tda p_{\ell, N}
        \end{bmatrix}\Bigg\Vert_2\leq C\tau\epsilon\Vert\bfa X\bfa X^\top\Vert_2^2.
    \end{align*}
    Then the rest of the proof focuses on showing that the rest of the terms are small. Note that using \eqref{diffhrpe1}, we show that
    \begin{align*}
        \lef\Vert\tda H^{rpe,1}-\bfa H^{rpe,1}\rig\Vert_2\leq\tau\epsilon\Vert\bfa X\bfa X^\top\Vert_2^2.
    \end{align*}
    And for the last term, we can show that
    \begin{align*}
        \Big\Vert\sum_{m\in[M]}\bfa V_m^{rpe,2}\tda H^{rpe,1}&\times\sigma\lef((\bfa K_m^{rpe,2}\tda H^{rpe,1})^\top(\bfa Q_m^{rpe,2}\tda H^{rpe,1})\rig)\\
        &-\sum_{m\in[M]}\bfa V_m^{rpe,2}\bfa H^{rpe,1}\times\sigma\lef((\bfa K_m^{rpe,2}\bfa H^{rpe,1})^\top(\bfa Q_m^{rpe,2}\bfa H^{rpe,1})\rig)\Big\Vert_2\\
        &\leq C\tau\epsilon\Vert\bfa X\bfa X^\top\Vert_2^2. 
    \end{align*}
    Collecting the above pieces, we finally show that
    \begin{align*}
        \Bigg\Vert\tda H^{rpe,2}-\begin{bmatrix}
            \bfa X\\
            \bfa X\bfa X^\top,\bfa 0\\
            \tda p_{2,1},\ldots,\tda p_{2,N}\\
            \tda p_{3,1},\ldots,\tda p_{3,N}\\
            \tda p_{3,1}^{(\tau)},\bfa 0\\
            \Vert\bfa X\bfa X^\top\tda p_{3,1}^{(\tau)}\Vert_2^{\frac{1}{2}}\tda p_{3,1}^{(\tau)},\bfa 0\\
            \tda p_{6,1},\ldots,\tda p_{6,N}\\
            \vdots\\
            \tda p_{\ell,1},\ldots,\tda p_{\ell,N}
        \end{bmatrix} \Bigg\Vert_2\leq C\tau\epsilon\Vert\bfa X\bfa X^\top\Vert_2^2.
    \end{align*}
    % \begin{align*}
    %     \Bigg\Vert\tda H^{rpe,2}-\begin{bmatrix}
    %         \bfa X\\
    %         \tda y\\
    %         \bfa X\bfa X^\top,\bfa 0\\
    %         \tda p_{2,1}\ldots,\tda p_{2,N}\\
    %         \tda p_{3,1}\ldots,\tda p_{3,N}\\
    %         \Vert\bfa X\bfa X^\top\tda p_{3,1}^{(\tau)}\Vert_2^{\frac{1}{2}}\tda p_{3,1}^{(\tau)},\bfa 0\\
    %         \bfa 0
    %     \end{bmatrix}\Bigg\Vert_2.
    % \end{align*}
    Then we construct another layer to remove the principal components from the matrix $\bfa X\bfa X^\top$, given by
    \begin{align*}
        &-\bfa V_1^{rpe,3}=\bfa V_2^{rpe,3}= \begin{bmatrix}
            \bfa 0_{(d+1)\times(4d+1)}&\bfa 0&\bfa 0\\
            \bfa 0& I_d&\bfa 0\\
            \bfa 0&\bfa 0&\bfa 0
        \end{bmatrix},\qquad\bfa Q_1^{rpe,3}=-\bfa Q_2^{rpe,3}=\begin{bmatrix}
            \bfa 0_{d\times(4d+1)}&I_d&\bfa 0\\
            \bfa 0&\bfa 0&\bfa 0
        \end{bmatrix},\\
        &\bfa K_1^{rpe,3}=\bfa K_2^{rpe,3}=\begin{bmatrix}
            \bfa 0_{d\times(4d+1)}& I_d&\bfa 0\\
            \bfa 0&\bfa 0&\bfa 0
        \end{bmatrix}.
    \end{align*}
    Then we can show that
    \begin{align*}
        (\bfa Q_1^{rpe,3}\tda H^{rpe,2})^\top =\begin{bmatrix}
            \Vert\bfa X\bfa X^\top\tda p_{3,1}^{(\tau)}\Vert_2^{\frac{1}{2}}\tda p_{3,1}^{(\tau),\top}&\bfa 0\\
            \bfa 0&\bfa 0
        \end{bmatrix},\qquad\bfa K_1^{rpe,3}\tda H^{rpe,2}=\begin{bmatrix}
            \bfa 0&\bfa 0\\
            I_d&\bfa 0\\
            \bfa 0&\bfa 0
        \end{bmatrix}.
    \end{align*}
    Then it is further noted that
    $
       -(\bfa Q_2^{rpe,3}\tda H^{rpe,2})^\top\bfa K_2^{rpe,3}\tda H^{rpe,2}= (\bfa Q_1^{rpe,3}\tda H^{rpe,2})^\top\bfa K_1^{rpe,3}\tda H^{rpe,2} 
    $ satisfies
    \begin{align*}
        \Bigg\Vert(\bfa Q_1^{rpe,3}\tda H^{rpe,2})^\top\bfa K_1^{rpe,3}\tda H^{rpe,2}-\begin{bmatrix}
            \Vert\bfa X\bfa X^\top\tda p_{3,1}^{(\tau)}\Vert_2^{\frac{1}{2}}\tda p_{3,1}^{(\tau),\top}&\bfa 0\\
            \bfa 0&\bfa 0
        \end{bmatrix}\Bigg\Vert_2\leq C\tau\epsilon\Vert\bfa X\bfa X^\top\Vert_2^2.
    \end{align*}
    And therefore, combining our construction for $\bfa V_m$, it is noted that
    \begin{align*}
        \Bigg\Vert\sum_{m=1}^2\bfa V_m\tda H^{rpe,2}\times\sigma((\bfa Q_1^{rpe,3}\tda H^{rpe,2})^\top\bfa K_1^{rpe,3}\tda H^{rpe,2})&-\begin{bmatrix}
            \bfa 0_{(d+1)\times N}\\
            -\Vert\bfa X\bfa X^\top\tda p_{3,1}^{(\tau)}\Vert_2\tda p_{3,1}^{(\tau)}\tda p_{3,1}^{(\tau),\top},\bfa 0\\
            \bfa 0
        \end{bmatrix}\Bigg\Vert_2\\
        &\leq C\tau\epsilon\Vert\bfa X\bfa X^\top\Vert_2^2.
    \end{align*}
    Therefore, we can further show that
    \begin{align*}
        \tda H^{rpe,3} =\tda H^{rpe,2}+ \sum_{m=1}^2\bfa V_{m}^{rpe,3}\tda H^{rpe,2}\times\sigma\lef((\bfa Q_m^{rpe,3}\tda H^{rpe,2})^\top\bfa K_m^{rpe,3}\tda H^{rpe,2}\rig)
    \end{align*}
    satisfies
    \begin{align*}
       \Bigg\Vert \tda H^{rpe,3}-\begin{bmatrix}
            \bfa X\\
            \bfa X\bfa X^\top-\Vert\bfa X\bfa X^\top\tda p_{3,1}^{(\tau)}\Vert_2\tda p_{3,1}^{(\tau)}\tda p_{3,1}^{(\tau),\top},\bfa 0\\
            \tda p_{2,1},\ldots,\tda p_{2,N}\\
            \tda p_{3,1},\ldots,\tda p_{3,N}\\
            \tda p_{3,1}^{(\tau)},\bfa 0\\
            \tda p_{5,1},\ldots,\tda p_{5,N}\\
            \vdots\\
            \tda p_{\ell,1},\ldots,\tda p_{\ell,N}
        \end{bmatrix}\Bigg\Vert_2\leq C\tau\epsilon\Vert\bfa X\bfa X^\top\Vert_2^2.
    \end{align*}
    And we can construct another layer to remove the term $\Vert\bfa X\bfa X^\top\tda p_{3,1}^{(\tau)}\Vert_2^{\frac{1}{2}}\tda p_{3,1}^{(\tau)}$, which is achieved by 
    \begin{align*}
        &-\bfa V_1^{rpe,4} = \bfa V_2^{rpe,4} =  \begin{bmatrix}
            \bfa 0_{(4d+1)\times(4d+1)}&\bfa 0&\bfa 0\\
            \bfa 0_{d\times(4d+1)}& I_d&\bfa 0\\
            \bfa 0&\bfa 0&\bfa 0
        \end{bmatrix},\\
        &\bfa Q_1^{rpe,4} = -\bfa Q_2^{rpe,4}=\begin{bmatrix}
            &\bfa 0_{(3d+1)\times D}&\\
            \bfa 0_{d\times (2d+1)}& I_d&\bfa 0\\
            &\bfa 0&
        \end{bmatrix},\\
        &\bfa K_1^{rpe,4}= \bfa K_2^{rpe,4} =\begin{bmatrix}
            &\bfa 0_{(3d+1)\times D}&\\
            \bfa 0_{d\times (2d+1)}& I_d&\bfa 0\\
            &\bfa 0&
        \end{bmatrix}.
    \end{align*}
    Using the above construction, we can further show that
    \begin{align*}
        \Bigg\Vert\tda H^{rpe,4}-\begin{bmatrix}
            \bfa X\\
            \bfa X\bfa X^\top-\Vert\bfa X\bfa X^\top\tda p_{3,1}^{(\tau)}\Vert_2\tda p_{3,1}^{(\tau)}\tda p_{3,1}^{(\tau),\top},\bfa 0\\
            \tda p_{2,1},\ldots,\tda p_{2,N}\\
            \tda p_{3,1},\ldots,\tda p_{3,N}\\
            \tda p_{3,1}^{(\tau)},\bfa 0\\
            \tda p_{5,1},\ldots,\tda p_{5,N}\\
            \vdots\\
            \tda p_{\ell,1},\ldots,\tda p_{\ell,N}
        \end{bmatrix}\Bigg\Vert_2\leq C\tau\epsilon\Vert\bfa X\bfa X^\top\Vert_2^2.
    \end{align*}
    Then we proceed to recover the rest of the $k$ principal eigenvectors using similar model architecture given by the ones used by the Power Iterations. For the computation over the $\tau$-th eigenvector, we denote $\tda H^{pow, \eta, 1}$ till $\tda H^{pow, \eta, \tau}$ to be the intermediate states corresponding to the $\eta$-th power iteration. We denote $\tda H^{rpe,\eta,\tau_0}$ to be the output of $\eta$-th removal of principal eigenvector layers for the $\tau$-th eigenvector. Furthermore, we iteratively define
    \begin{align*}
        \bfa A_1 =\bfa X\bfa X^\top-\Vert\bfa X\bfa X^\top\tda p_{3,1}^{(\tau)}\Vert_2\tda p_{3,1}^{(\tau)}\tda p_{3,1}^{(\tau),\top},\qquad \bfa A_{i+1}=\bfa A_{i}-\Vert\bfa A_i\tda p_{3,i}^{(\tau)}\Vert_2\tda p_{3,i}^{(\tau)}\tda p_{3,i}^{(\tau),\top},\qquad\forall i\in[k].
    \end{align*}
    Then, applying the subadditivity of the $2$-norm, we can show that
    \begin{align*}
        \Bigg\Vert\tda H^{rpe,4,k}-\begin{bmatrix}
            \bfa X\\
            \bfa A_{k+1},\bfa 0\\
            \tda p_{2,1},\ldots,\tda p_{2,N}\\
            \tda p_{3,1},\ldots,\tda p_{3,N}\\
            \tda p_{3,1}^{(\tau)},\bfa 0\\
            \tda p_{3,2}^{(\tau)},\bfa 0\\
            \vdots\\
            \tda p_{3,k}^{(\tau)},\bfa 0
        \end{bmatrix}\Bigg\Vert_2\leq C\tau k\epsilon\Vert\bfa X\bfa X^\top\Vert_2^2.
    \end{align*}
    For simplicity, we denote $\tda A=\begin{bmatrix}
        \bfa X\\
        \bfa A_{k+1},\bfa 0\\
        \tda p_{2,1},\ldots,\tda p_{2,N}\\
        \tda p_{3,1},\ldots,\tda p_{3,N}
    \end{bmatrix}$ and $\tda P=\begin{bmatrix}
        \tda p_{3,1}^{(\tau)}\\
        \tda p_{3,2}^{(\tau)}\\
        \vdots\\
        \tda p_{3,k}^{(\tau)}
    \end{bmatrix}$ from here. 
    \begin{center}
        \textbf{4. Finishing Up.}
    \end{center}
    The finishing-up phase considers constructing $\tda W_0$ and $\tda W_1$ that adjust the final output format. Our construction gives the following 
    \begin{align*}
        \tda W_0 = \begin{bmatrix}
            \bfa 0,I_{kd}
        \end{bmatrix},\qquad\tda W_1=\begin{bmatrix}
            1\\
            \bfa 0_{N-1}
        \end{bmatrix}.
    \end{align*}
    And we can show that
    \begin{align*}
        \Bigg\Vert\tda W_0\tda H^{rpe,4,k}\tda W_1-\begin{bmatrix}
            \tda p_{3,1}^{(\tau)}\\
            \tda p_{3,2}^{(\tau)}\\
            \vdots\\
            \tda p_{3,k}^{(\tau)}
        \end{bmatrix}\Bigg\Vert_2\leq C\tau k\epsilon\Vert\bfa X\bfa X^\top\Vert_2^2.
    \end{align*}
        We further use the result given by lemma \ref{lm3.2}, denote $a_{\eta}:=\lef\Vert\bfa v_{\eta}-\tda p_{3,\eta}^{(\tau)}\rig\Vert_2$, $\wh\lambda_{\eta}=\lef\Vert \bfa A_{\eta}\tda p_{3,\eta}^{(\tau)}\rig\Vert_2$, and $b_{\eta}:=|\lambda_{\eta}-\wh \lambda_{\eta}|$ for $\eta\in[k]$, we obtain that for all $\eta\geq 1$, given the number of iterations $\tau\geq C\frac{\log(1/\epsilon_0\delta)}{2\epsilon_0}$ where the constant value $C$ depends on $d$,
    \begin{align*}
    a_{\eta+1}\leq\frac{\max_{i\in[\eta]}b_{i}+\sum_{i=1}^{\eta}2\lambda_i a_i}{\Delta},\qquad b_{\eta+1}\leq\frac{2\lambda_{\eta+1}}{\Delta}\bl\max_{i\in[\eta]}b_{\eta}+\sum_{i=1}^{\eta} 2\lambda_ia_i\br+\lambda_{\eta+1}\sqrt{2\epsilon_0}.
    \end{align*}
    Further, note that the starting point is given by
    $a_{1}\leq \sqrt{2\epsilon_0}$, $b_1\leq\lambda_{1}\sqrt{2\epsilon_0}$. Introducing $A_{\eta}=\sum_{i=1}^{\eta} 2\lambda_ia_i$, we obtain that
$        A_{\eta+1} =\sum_{i=1}^{\eta+1}2\lambda_ia_i = A_{\eta}+2\lambda_{\eta+1}a_{\eta+1}$ which alternatively implies that
    \begin{align*}
        \frac{1}{2\lambda_{\eta+1}}(A_{\eta+1}-A_{\eta})\leq\frac{\max_{i\in[\eta]}b_i+A_{\eta}}{\Delta},\qquad b_{\eta+1}\leq\frac{2\lambda_{\eta+1}}{\Delta}\bl\max_{i\in[\eta]}b_{\eta}+A_{\eta}\br+\lambda_{\eta+1}\sqrt{2\epsilon_0}.
    \end{align*}
    We use the fact 
        $\frac{\lambda_{\eta}}{\Delta}>1$ for all $\eta\in[k]$
    to show the following
    \begin{align*}
A_{\eta+1}+\max_{i\in[\eta+1]}b_i\leq\frac{5\lambda_{\eta+1}}{\Delta}\lef(A_{\eta}+\max_{i\in[\eta]} b_i\rig)+\lambda_1\sqrt{2\epsilon_0}, \qquad A_1+b_1=2\lambda_1\sqrt{2\epsilon_0},
    \end{align*}
    which implies that
    \begin{align}\label{iterativeeq}
    A_{\eta+1}+\max_{i\in[\eta+1]}b_i+&\frac{\lambda_1\sqrt{2\epsilon_0}}{\frac{5\lambda_{1}}{\Delta}-1}\leq\frac{5\lambda_{1}}{\Delta}\bl A_{\eta}+\max_{i\in[\eta]}b_i +\frac{\lambda_1\sqrt{2\epsilon_0}}{\frac{5\lambda_{1}}{\Delta}-1}\br,\nnb\\
        A_{\eta+1}+\max_{i\in[\eta+1]}b_i+&\frac{\lambda_1\sqrt{2\epsilon_0}}{\frac{5\lambda_{1}}{\Delta}-1}\leq\bl A_1+b_1+\frac{\lambda_1\sqrt{2\epsilon_0}}{\frac{5\lambda_1}{\Delta}-1}\br\prod_{i=1}^{\eta}\bl\frac{5\lambda_{i+1}}{\Delta}\br\nnb\\
        &=\lambda_1\sqrt{2\epsilon_0}\bl 2+\frac{1}{\frac{5\lambda_1}{\Delta}-1} \br\prod_{i=1}^{\eta}\bl\frac{5\lambda_{i+1}}{\Delta}\br.
    \end{align}
    Therefore, applying the inequality given by \eqref{iterativeeq} we can show that, for $\eta\leq k$, we have for all $\eta\in[k-1]$,
    \begin{align*}
        a_{\eta+1}&\leq\frac{1}{\Delta}\bl \lambda_1\sqrt{2\epsilon_0}\bl 2+\frac{1}{\frac{5\lambda_1}{\Delta}-1}\br\prod_{i=1}^{\eta}\bl\frac{5\lambda_{i+1}}{\Delta}\br-\frac{\lambda_1\sqrt{2\epsilon_0}}{\frac{5\lambda_1}{\Delta}-1}\br,\\
        b_{\eta+1}&\leq\frac{2\lambda_{\eta}\lambda_1\sqrt{2\epsilon_0}}{\Delta}\bl 2+\frac{1}{\frac{5\lambda_1}{\Delta}-1}\br\prod_{i=1}^{\eta}\bl\frac{5\lambda_{i+1}}{\Delta}\br+\lambda_{\eta+1}\sqrt{2\epsilon_0}.
    \end{align*}
    Therefore collecting pieces, we conclude that there exists a transformer with a number of layers $2\tau+4k+1$ and a number of heads $M\leq \lambda_1^d\frac{C(d)}{\epsilon^2}$ such that
    the final output $\wha v_1,\ldots,\wha v_{k}$ given by the Transformer model satisfy $\forall \eta\in[k-1]$,
    \begin{align*}
        \lef\Vert\wha v_{\eta+1}-\bfa v_{\eta+1}\rig\Vert_2\leq C\tau \epsilon\lambda_1^2+\frac{1}{\Delta}\bl\lambda_1\sqrt{2\epsilon_0}\bl 2+\frac{1}{\frac{5\lambda_1}{\Delta}-1}\br\prod_{i=1}^{\eta}\bl\frac{5\lambda_{i+1}}{\Delta}\br-\frac{\lambda_1\sqrt{2\epsilon_0}}{\frac{5\lambda_1}{\Delta}-1}\br.
    \end{align*}
    And the rest of the result directly follows.
    \end{proof}

    \subsection{Proof of Lemma \ref{lm3.1}}
        \begin{proof}
        To prove the above result, we consider two events
$            A_1 =\lef\{\Vert \bfa y\Vert_2\geq \sqrt{\frac{1}{\epsilon}}\rig\}$, $A_2=\lef\{|\bfa y^\top\bfa v|\leq \sqrt{\epsilon}\rig\}$, then we can show that
        \begin{align*}
           \lef\{ |\bfa v^\top\bfa x|\leq\frac{1}{\sqrt\epsilon}\rig\}\subset A_1\cup A_2\quad\Rightarrow\quad\bb P\bl|\bfa v^\top\bfa x|\leq\sqrt{\epsilon}\br\leq\bb P(A_1)+\bb P(A_2).
        \end{align*}
        And we use the tail bound for Chi-square given by \citep{laurent2000adaptive} to obtain that as $\epsilon<d^{-1}$,
        \begin{align*}
            \bb P(A_1) = \bb P\lef(\Vert\bfa y\Vert_2^2\geq \epsilon^{-1}\rig)\leq\exp\lef(-C\epsilon^{-1}\rig).
        \end{align*}
        Similarly, consider the event $A_2$, note that $\bfa y^\top\bfa v\sim N(0,1)$, we use the cdf of the folded normal distribution to obtain that
        \begin{align*}
            \bb P\lef(A_2\rig) = \bb P\lef(\lef|\bfa v^\top\bfa y\rig|\leq\sqrt{\epsilon}\rig)=erf\lef(\frac{\sqrt\epsilon}{\sqrt 2}\rig)=\frac{2}{\sqrt{\pi}}\bl \sqrt\epsilon-\frac{(\sqrt\epsilon)^3}{3}+\frac{(\sqrt\epsilon)^5}{10}-\frac{(\sqrt\epsilon)^7}{42}\br\leq\frac{\sqrt\epsilon}{\sqrt{\pi}}.
        \end{align*}
        Then we obtain that 
        \begin{align*}
            \bb P\bl|\bfa v^\top\bfa x|\leq\sqrt\epsilon\br\leq \frac{\sqrt\epsilon}{\sqrt{\pi}}+\exp\lef(-C\epsilon^{-1}\rig).
        \end{align*}
        Consider in total of $k$ independent random vectors $\bfa x_1,\ldots,\bfa x_k$, and arbitrary $k$ vectors $\bfa v_1,\ldots,\bfa v_k$, we can show that
        \begin{align*}
            \bb P\bl\exists i\text{ such that }&\bfa x_i^\top\bfa v_i\leq\epsilon\br\leq k\bb P\bl\bfa x_1^\top\bfa v_1\leq\epsilon\br\leq\frac{k\sqrt{\epsilon}}{\sqrt{\pi}}+k\exp(-C\epsilon^{-1}).
        \end{align*}
    \end{proof}

\subsection{Proof of Lemma \ref{lm3.2}}

\begin{lemma}\label{lm3.2}
Assume that the correlation matrix $\bfa X\bfa X^\top$ has eigenvalues $\lambda_1>\lambda_2>\ldots>\lambda_{k}$. Assume that the eigenvectors are given by $\bfa v_1,\bfa v_2,\ldots,\bfa v_n$ and the eigenvalues satisfy $\inf_{i\neq j}|\lambda_i-\lambda_j|=\Delta$. Then, given that the estimate for the first $\tau$ eigenvectors satisfy
$    \bfa v_i^\top\wha v_i\geq 1-\epsilon_i $ and the eigenvalues satisfy $|\lambda_i-\wh\lambda_i|\leq\delta_i$, the principal eigenvector of $\bfa X\bfa X^\top-\sum_{i=1}^{\tau}\wh\lambda_i\wha v_i\wha v_i^\top$ denoted by $\tda v_{\tau+1}$ satisfies
\begin{align*}
    \Vert\tda v_{\tau+1}-\bfa v_{\tau+1}\Vert_2 \leq\frac{\max_{i\in[\tau]}\delta_i+\sum_{i=1}^\tau\sqrt8\lambda_i\sqrt{\epsilon_i}}{\Delta}.
\end{align*}
Alternatively, we can also show that the eigenvector $\wha v_{\tau+1}$ returned by power method with $k= \frac{\log(1/\epsilon_0\delta)}{2\epsilon_0}$ that is initialized by  satisfies
\begin{align*}
    \wha v_{\tau+1}^\top\bfa v_{\tau+1} \geq 1-\epsilon_{\tau+1}:=  1-\frac{1}{2}\Big(\frac{\max_{i\in[\tau]}\delta_i+\sum_{i=1}^{\tau}\sqrt{8}\lambda_i\sqrt{\epsilon_i}}{\Delta}+\sqrt{2\epsilon_0}\Big)^2,
\end{align*}
\end{lemma}
    \begin{proof}
    Our proof is given by inductive arguments. Consider our obtained estimates $\{\wha v_i\}_{i\in[k]}$ for the eigenvectors $\{\bfa v_i\}_{i\in[k]}$ satisfy
    \begin{align*}
        \bfa v_i^\top\wha v_i\geq 1-\epsilon_i\qquad \forall i\in[\tau],\qquad|\lambda_i-\wh\lambda_i|\leq\delta_i.
    \end{align*}
    We note that for the eigenvectors, we have for a vector $\bfa v_0$,
    \begin{align*}
        \Vert\bfa v_i\bfa v_i^\top-\wha v_i\wha v_i^\top\Vert_2&=\sup_{\bfa v_0\in\bb S^{d-1}}\bfa v_0^\top(\bfa v_i\bfa v_i^\top-\wha v_i\wha v_i^\top)\bfa v_0=\sup_{\bfa v_0\in\bb S^{d-1}}(\bfa v_0^\top\bfa v_i)^2-(\bfa v_0^\top\wha v_i)^2\\
        &=\sup_{\bfa v_0\in\bb S^{d-1}}(\bfa v_0^\top(\bfa v_i-\wha v_i))(\bfa v_0^\top(\bfa v_i+\wha v_i^\top))\\
        &\leq 2\Vert\bfa v_i-\wha v_i\Vert_2=2\sqrt{\Vert\bfa v_i-\wha v_i\Vert_2^2} = 2\sqrt{\Vert\bfa v_i\Vert_2^2+\Vert\wha v_i\Vert_2^2-2\bfa v_i^\top\wha v_i} = 2\sqrt{2\epsilon_i}.
    \end{align*}
    Then, we can show by the subadditivity of the spectral norm,
    \begin{align*}
        \Big\Vert\bfa X\bfa X^\top-\sum_{i=1}^\tau\wh\lambda_i\wha v_i\wha v_i^\top\Big\Vert_2&=\Big\Vert\sum_{i=1}^k\lambda_i\bfa v_i\bfa v_i^\top-\sum_{i=1}^{\tau}\wh\lambda_i\wha v_i\wha v_i^\top\Big\Vert_2\\
        &\leq\Big\Vert\sum_{i=1}^k\lambda_i\bfa v_i\bfa v_i^\top-\sum_{i=1}^\tau\lambda_i\wha v_i\wha v_i^\top\Big\Vert_2+\Big\Vert\sum_{i=1}^{\tau}\delta_i\wha v_i\wha v_i^\top\Big\Vert_2\\
        &\leq\Big\Vert\sum_{i=\tau+1}^k\lambda_i\bfa v_i\bfa v_i^\top\Big\Vert_2+\Big\Vert\sum_{i=1}^\tau\delta_i\wha v_i\wha v_i^\top\Big\Vert_2+\Big\Vert\sum_{i=1}^{\tau}\lambda_i\bfa v_i\bfa v_i^\top-\sum_{i=1}^{\tau}\lambda_i\wha v_i\wha v_i^\top \Big\Vert_2\\
        &\leq\lambda_{\tau+1} + \max_{i\in[\tau]}\delta_i+ \Big\Vert\sum_{i=1}^{\tau}\lambda_i(\bfa v_i\bfa v_i^\top-\wha v_i\wha v_i^\top)\Big\Vert_2 \\
        &\leq\lambda_{\tau+1}+\max_{i\in[\tau]}\delta_i+\sum_{i=1}^{\tau}\lambda_i\Big\Vert\bfa v\bfa v_i^\top-\wha v_i\wha v_i^\top\Big\Vert_2\\
        &\leq\lambda_{\tau+1}+\max_{i\in[\tau]}\delta_i+\sum_{i=1}^{\tau}\sqrt{8}\lambda_i\sqrt{\epsilon_i}.
    \end{align*}
    By a similar argument, we can also show that
    \begin{align*}
        \Big\Vert\bfa X\bfa X^\top-\sum_{i=1}^{\tau}\wh\lambda_i\wha v_i\wha v_i^\top\Big\Vert_2\geq\lambda_{\tau+1}-\max_{i\in[\tau]}\delta_i-\sum_{i=1}^{\tau}\sqrt 8\lambda_i\sqrt{\epsilon_i}.
    \end{align*}
    To study the convergence of the eigenvectors, we notice that by Davis-Kahan Theorem by \citep{yu2015useful} we can show that the principal eigenvector $\tda v_{\tau+1}=\argmax_{\bfa v\in\bb S^{d-1}}$ satisfies
    \begin{align*}
        \Vert\tda v_{\tau+1}-\bfa v_{\tau+1}\Vert_2\leq\frac{\Big|\lef\Vert\bfa X\bfa X^\top-\sum_{i}^{\tau}\wh\lambda_i\wha v_i\wha v_i^\top\rig\Vert-\lambda_{\tau+1}\Big|}{\max\{|\lambda_{\tau+1}-\lambda_{\tau}|,|\lambda_{\tau-1}-\lambda_{\tau}|\}}\leq\frac{\max_{i\in[\tau]}\delta_i+\sum_{i=1}^{\tau}\sqrt 8\lambda_i\sqrt{\epsilon_i}}{\Delta}.
    \end{align*}
    % Alternatively, we can show that
    % \begin{align*}
    %     \tda v_{\tau+1}^\top\bfa v_{\tau+1}=\frac{1}{2}\lef(2-\Vert\tda v_{\tau+1}-\bfa v_{\tau+1}\Vert_2^2\rig)=1-\Big(\frac{\max_{i\in[\tau]}\delta_i+\sum_{i=1}^{\tau}\sqrt 8\lambda_i\sqrt{\epsilon_i}}{2\Delta}\Big)^2.
    % \end{align*}
    Considering the eigenvector returned by the power method, we can show by the subadditivity of $L_2$ norm, we obtain that $\Vert\wha v_{\tau+1}-\bfa v_{\tau+1}\Vert_2\leq \Vert\tda v_{\tau+1}-\wha v_{\tau+1}\Vert_2+\Vert\tda v_{\tau+1}-\bfa v_{\tau+1}\Vert_2\leq \frac{\max_{i\in[\tau]}\delta_i+\sum_{i=1}^{\tau}\sqrt{8}\lambda_i\sqrt{\epsilon_i}}{\Delta}+\sqrt{2\epsilon_0}$
    \begin{align*}
        \wha v_{\tau+1}^\top\bfa v_{\tau+1}&=\frac{1}{2}\lef(2-\Vert\bfa v_{\tau+1}-\wha v_{\tau+1}\Vert_2^2\rig)\geq\frac{1}{2}\lef(2-\lef(\Vert\tda v_{\tau+1}-\wha v_{\tau+1}\Vert_2+\Vert\bfa v_{\tau+1}-\tda v_{\tau+1}\Vert_2\rig)^2\rig)\\
        &=1-\frac{1}{2}\Big(\frac{\max_{i\in[\tau]}\delta_i+\sum_{i=1}^{\tau}\sqrt{8}\lambda_i\sqrt{\epsilon_i}}{\Delta}+\sqrt{2\epsilon_0}\Big)^2.
    \end{align*}
    Moreover, considering the estimate of the eigenvalue, we have 
    \begin{align*}
        &\Big\Vert\Big(\bfa X\bfa X^\top -\sum_{i=1}^{\tau}\wh\lambda_i\wha v_i\wha v_i^\top\Big)\wha v_{\tau+1}\Big\Vert_2\\
        &\leq\Big\Vert\Big(\bfa X\bfa X^\top-\sum_{i=1}^{\tau}\lambda_i\bfa v_i\bfa v_i^\top\Big)\wha v_{\tau+1}\Big\Vert_2+\Big\Vert\sum_{i=1}^\tau\lambda_i\bfa v_i\bfa v_i^\top-\sum_{i=1}^{\tau}\wh\lambda_i\wha v_i\wha v_i^\top \Big\Vert_2\\
        &\leq \Big\Vert\Big(\bfa X\bfa X^\top-\sum_{i=1}^{\tau}\lambda_i\bfa v_i\bfa v_i^\top\Big)\wha v_{\tau+1} \Big\Vert_2+\Big\Vert\sum_{i=1}^{\tau}\lambda_i\bfa v_i\bfa v_i^\top-\sum_{i=1}^{\tau}\lambda_i\wha v_i\wha v_i^\top\Big\Vert_2+\Big\Vert \sum_{i=1}^{\tau}\lef(\lambda_i-\wh\lambda_i\rig)\wha v_i\wha v_i^\top\Big\Vert_2\\
        &\leq\Big\Vert\Big(\bfa X\bfa X^\top-\sum_{i=1}^{\tau}\lambda_i\bfa v_i\bfa v_i^\top\Big)\bfa v_{\tau+1}\Big\Vert_2+\Big\Vert\Big(\bfa X\bfa X^\top-\sum_{i=1}^{\tau}\lambda_i\bfa v_i\bfa v_i^\top\Big)\Big\Vert_2\Vert\wha v_{\tau+1}-\bfa v_{\tau+1}\Vert_2\\
        &+\max_{i\in[\tau]}\delta_i+\sum_{i=1}^{\tau}\sqrt{8}\lambda_i\sqrt{\epsilon_i}\\
        &=\lambda_{\tau+1}+\lambda_{\tau+1}\Big(\frac{\max_{i\in[\tau]}\delta_i+\sum_{i=1}^{\tau}\sqrt 8\lambda_i\sqrt{\epsilon_i}}{\Delta}+\sqrt{2\epsilon_0}\Big)+\max_{i\in[\tau]}\delta_i+\sum_{i=1}^{\tau}\sqrt 8\lambda_i\sqrt{\epsilon_i}.
    \end{align*}
    Therefore, by similar arguments, we can show that
    \begin{align*}
        \Big|\Big\Vert \Big(\bfa X\bfa X^\top-\sum_{i=1}^{\tau}\wh\lambda_i\wha v_i\wha v_i^\top\Big)\wha v_{\tau+1}\Big\Vert_2-\lambda_{\tau+1}\Big|\leq \frac{2\lambda_{\tau+1}}{\Delta}\Big(\max_{i\in[\tau]}\delta_i+\sum_{i=1}^{\tau}\sqrt{8}\lambda_i\sqrt{\epsilon_i}\Big)+\lambda_{\tau+1}\sqrt{2\epsilon_0}.
    \end{align*}
\end{proof}

\subsection{Proof of Lemma \ref{reluapprox}}

    \begin{lemma}[Approximation of norm by sum of Relu activations by Transformer networks]\label{reluapprox}
    Assume that there exists a constant $C$ with $\Vert\bfa v\Vert_2\leq C$. There exists a multi-head Relu attention layer with a number of heads $M>\lef(\frac{\overline R}{\underline R}\rig)^d\frac{C(d)}{\epsilon^2}\log(1+C/\epsilon)$ such that there exists $\{\bfa a_m\}_{m\in[M]}\subset\bb S^{N-1}$ and $\{c_m\}_{m\in[M]}\subset\bb R$ where for all $\bfa v$ with $\overline R\geq\Vert\bfa v\Vert_2\geq \underline R$, we have 
    \begin{align*}
        \bigg|\sum_{m=1}^Mc_m\sigma(\bfa a_m^\top\bfa v)-\frac{1}{\Vert\bfa v\Vert_2}+1\bigg|\leq\epsilon.
    \end{align*}
    Similarly, there exists a multi-head Relu attention layer with number of heads $M\leq\overline R^{\frac{d}{2}}\frac{C(d)}{\epsilon^2}\log\lef(1+C/\epsilon\rig)$, a set of vectors $\{\bfa b_m\}_{m\in[M]}\subset\bb S^{N-1}$ and $\{d_m\}_{m\in[M]}\subset\bb R$ such that 
    \begin{align*}
        \Big|\sum_{m=1}^Md_m\sigma(\bfa b_m^\top\bfa v)-\Vert\bfa v\Vert_2^{1/2}+1\Big|\leq\epsilon.
    \end{align*}
\end{lemma}

\begin{proof}
    Consider a set $\msf C^d(\overline R) :=\msf B^d_{\infty}(\overline R)\setminus\msf B_{2}^d(\underbar R)$, then it is not hard to check that given $\Vert\bfa v\Vert_2>C$ with some $C(d)>0$ depending on $d$ such that we have
    \begin{align*}
        \sup_{\bfa v\in\msf C^d(\overline R)}\pta_{v_{j_1},\ldots,v_{j_i}\in[d]}\bl\frac{1}{\Vert\bfa v\Vert_2}\br\leq\frac{C(d)}{\Vert\bfa v\Vert_2^d}\leq\frac{C(d)}{\underline R^d}.
    \end{align*}
    Therefore, consider the definition \ref{def6}, we have $C_{\ell}=\lef(\frac{\overline R}{\underline R}\rig)^d C(d)$.  Note that by proposition A.1 in \citep{bai2024transformers} shows that for a function that is $(R,C_{\ell})$ smooth with $R\geq 1$ is $(\epsilon_{approx}, R, M,C)$ approximable with $M\leq C(d)C_{\ell}\log(1+C_{\ell}/\epsilon_{approx})/\epsilon_{approx}^2$, we complete the proof. 

    Then we consider the function $\Vert\bfa v\Vert_2^{\frac{1}{2}}$, note that
    \begin{align*}
        \sup_{\bfa v\in\msf C^d(\overline R)}\pta_{v_{j_1},\ldots,v_{j_i}\in[d]}\Vert\bfa v\Vert_2^{\frac{1}{2}}\leq C\Vert\bfa v\Vert_2^{-\frac{1}{2}}\leq C\overline R^{-\frac{1}{2}}.
    \end{align*}
    And the rest of the proof follows similarly to the previous step.
\end{proof}

\clearpage

\section{Experimental Details}\label{sec:exp_details}

\subsection{Setup.}
We run all our experiments on RTX 2080 Ti GPUs.
We use PyTorch to construct our models and training process.
We use sklearn for data generation.
A training process with 2k steps roughly takes $0.5$ hours.

% Finally, we test our framework on two real-world datasets instead of the synthetic data generated from a multivariate Gaussian distribution.
% We train the model to predict top-$5$ eigenvalues and top-$1 \sim 5$ eigenvectors, with the former using a small model and the latter using a large model.

\subsection{Data.}\label{appendix:data}
\paragraph{Synthetic Dataset.}
For each $\bfa X_i \in \R^D$, we sample $Z_i \sim N(0, I) \in \R^D$.
We then form $Z = [Z_1, \cdots, Z_N]$ and transform it using an invertible matrix $L \sim N(0, I) \in \R ^{D \times D}$, yielding the desired training sample $\bfa X$.
To speed up the training process, we set $N < D$ in all our experiment settings.
With this design, the rank of the covariance matrix  $\bfa X^T X$ is at most $N$, meaning there are at least $D-N$ zero eigenvalues.
The eigenvectors corresponding to these zero eigenvalues are less meaningful.
Thus, to ensure predictions focus on meaningful eigenvectors, we increase $N$ to $10$ when predicting multiple eigenvectors.
We also adjust the data generation process to ensure the magnitude of eigenvalue across different $D$ to be at a similar level.

\paragraph{Real-world Dataset.}
For both the MNIST and FMNIST, we first normalize the images to zero mean.
Next, we perform SVD to extract the top-$D$ principal components and project the data onto these components, reducing feature dimension to $D = 10, 20$, and use $N = 10, 50$ for eigenvalue and eigenvector prediction respectively.
Last, we rescale the resulting matrix to ensure its magnitude is roughly the same level as training data (transformers are trained on synthetic data).
The rescaling process is critical to transformers as some images after SVD contain entries as large as $7e3$.
This will largely degrade the transformer's performance as it changes the input domain by a large margin.

% We start by verifying the simpler case with $N=5$ and predicting top-1 eigenvalue and eigenvector, with $D = 5, 10, 30, 50$.
% We then proceed to the harder case with $N=10$ and predict the top-$5$ eigenvalues and eigenvectors.

% and use Adam optimizer with batch size $64$ and learning rate $= 0.001$.
% If not specified, all the experiments is trained for 20k steps, except the multiple eigenvectors prediction experiment in section \ref{sec:eigvec_pred}.

\subsection{Hyperparameters.}
We list the hyperparameters in our experiments as below (table~\ref{table:data-param}).
We separate the hyperparameters used in predicting (1) eigenvalues and single eigenvectors, and (2) multiple eigenvectors.

\begin{table}[h]
        \centering
        \caption{Hyperparameters for Eigenvalue and Eigenvector Prediction.
        }
        % \resizebox{ \textwidth}{!}{  
        \begin{tabular}{l*{4}{c}}
        \toprule
            \bf{parameter} & $N=5$ & $N=10$  & $N=20$ \\ 
            \midrule
             steps (eigenvalue) & 20k & 20k & 20k \\
             steps (eigenvector) & 20k & 20k & 60k \\
            learning rate  & $1\text{e-}3$ & $5\text{e-}3$ & $5\text{e-}3$ \\
            Optimizer  & Adam & Adam & Adam \\
            batch size  & $64$ & $64$ & $64$  \\
            number of layers & $3$ & $3$ & $3$  \\
            hidden dimension & $64$ & $64$& $64$ \\
            number of heads  & $2$ & $2$& $2$ \\
            \bottomrule
        \end{tabular}
        \label{table:data-param}
    \end{table}

\subsection{Additional Experimental Results}\label{sec:add_exp}

% \paragraph{Evidence of the challenge of predicting high-order eigenvalue.} xxx.

% \paragraph{Convergence Results.}
% We include the training loss curve of all the experiments using synthetic datasets in the figure \ref{fig:loss}.
% All the loss is 

\begin{figure}[!h]
    \centering
    \minipage{0.3\textwidth}
        \includegraphics[width=\linewidth]{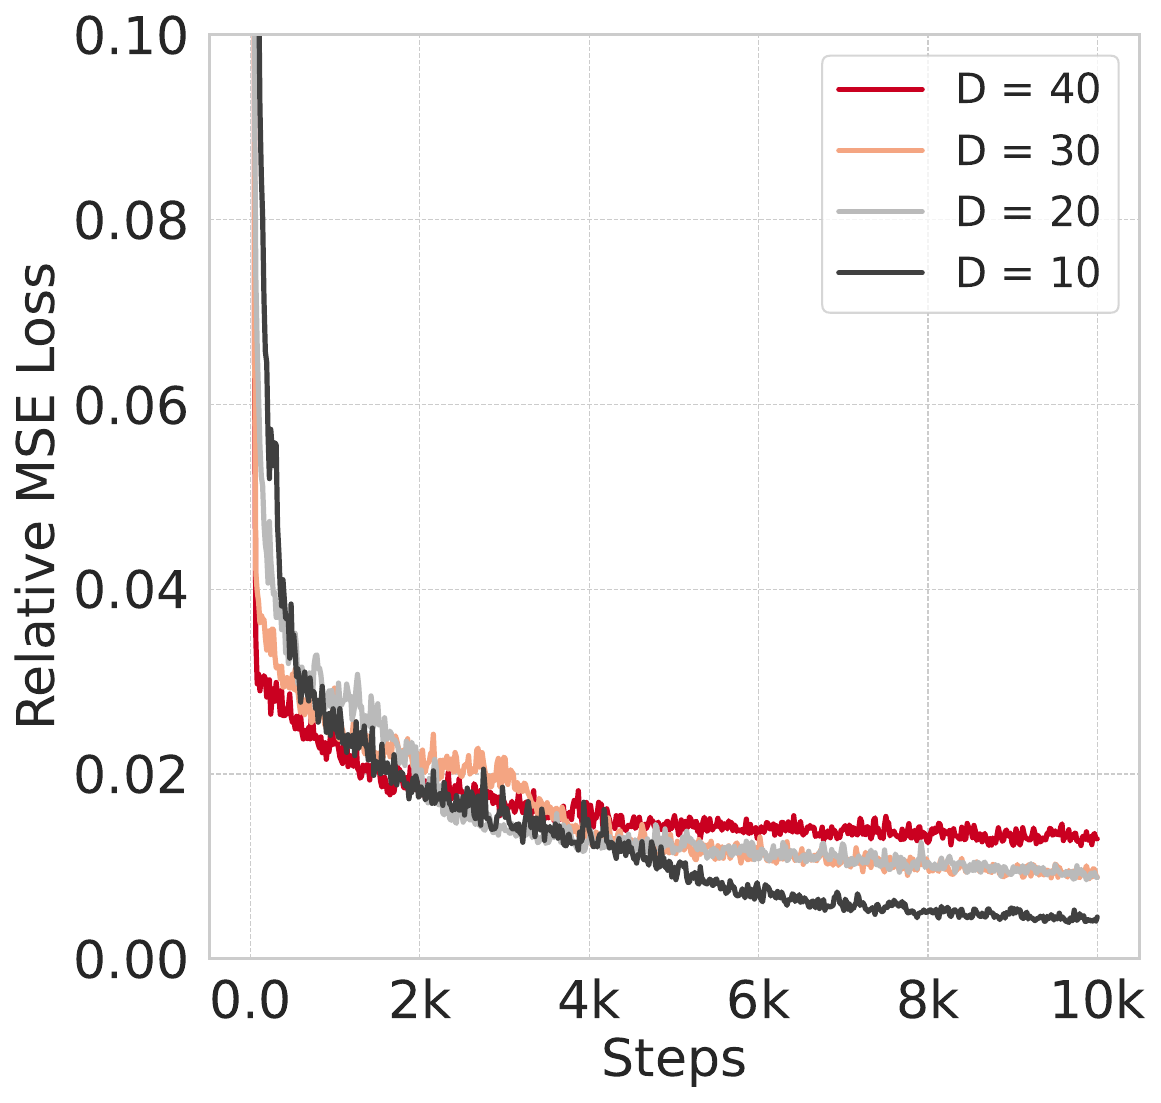}
    \endminipage\hfill
    \minipage{0.3\textwidth}
        \includegraphics[width=\linewidth]{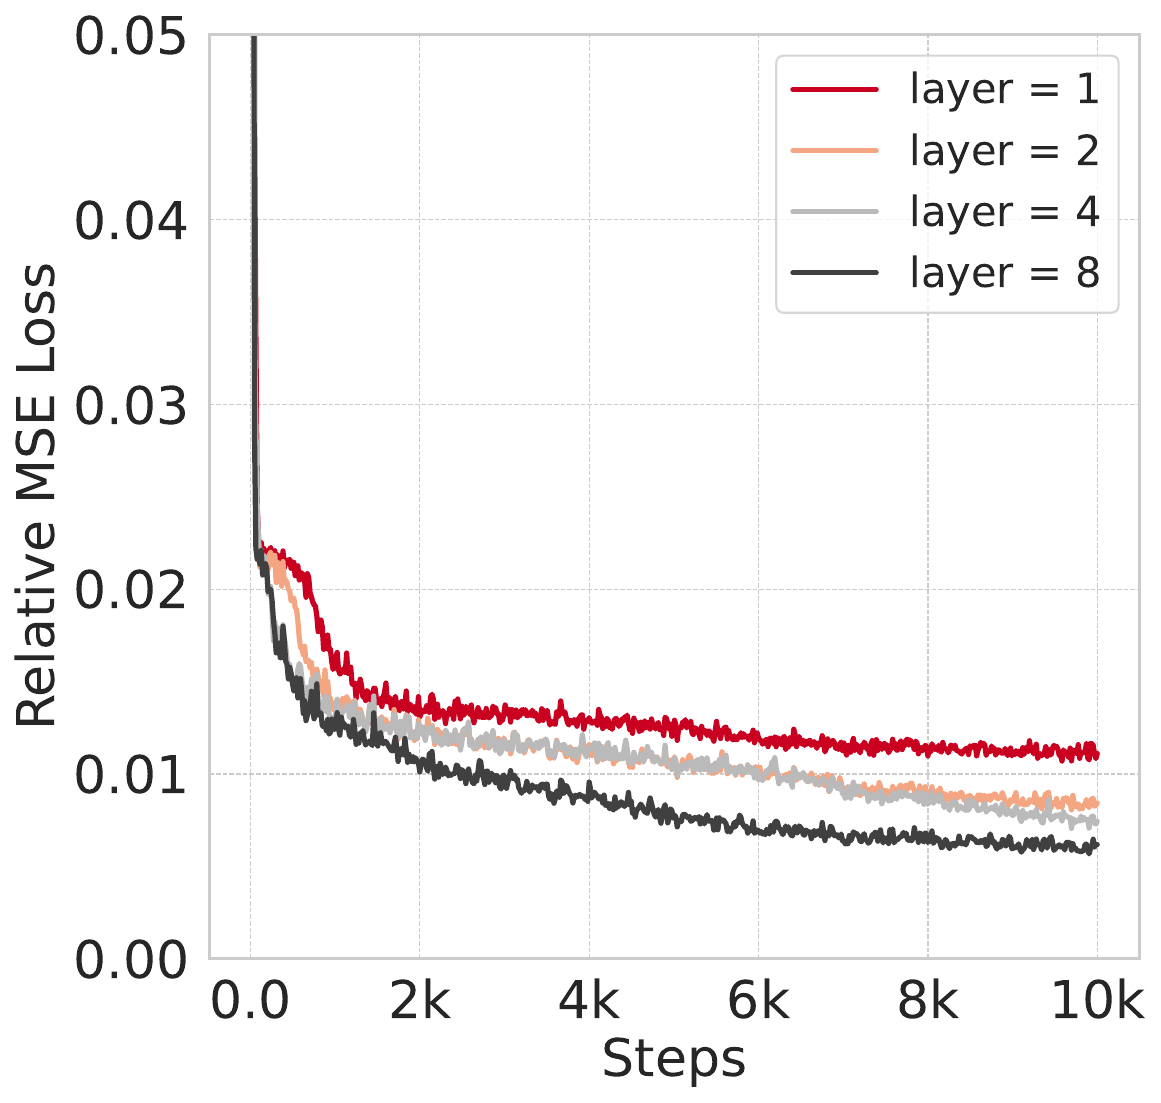}
    \endminipage\hfill
    \minipage{0.3\textwidth}
        \includegraphics[width=\linewidth]{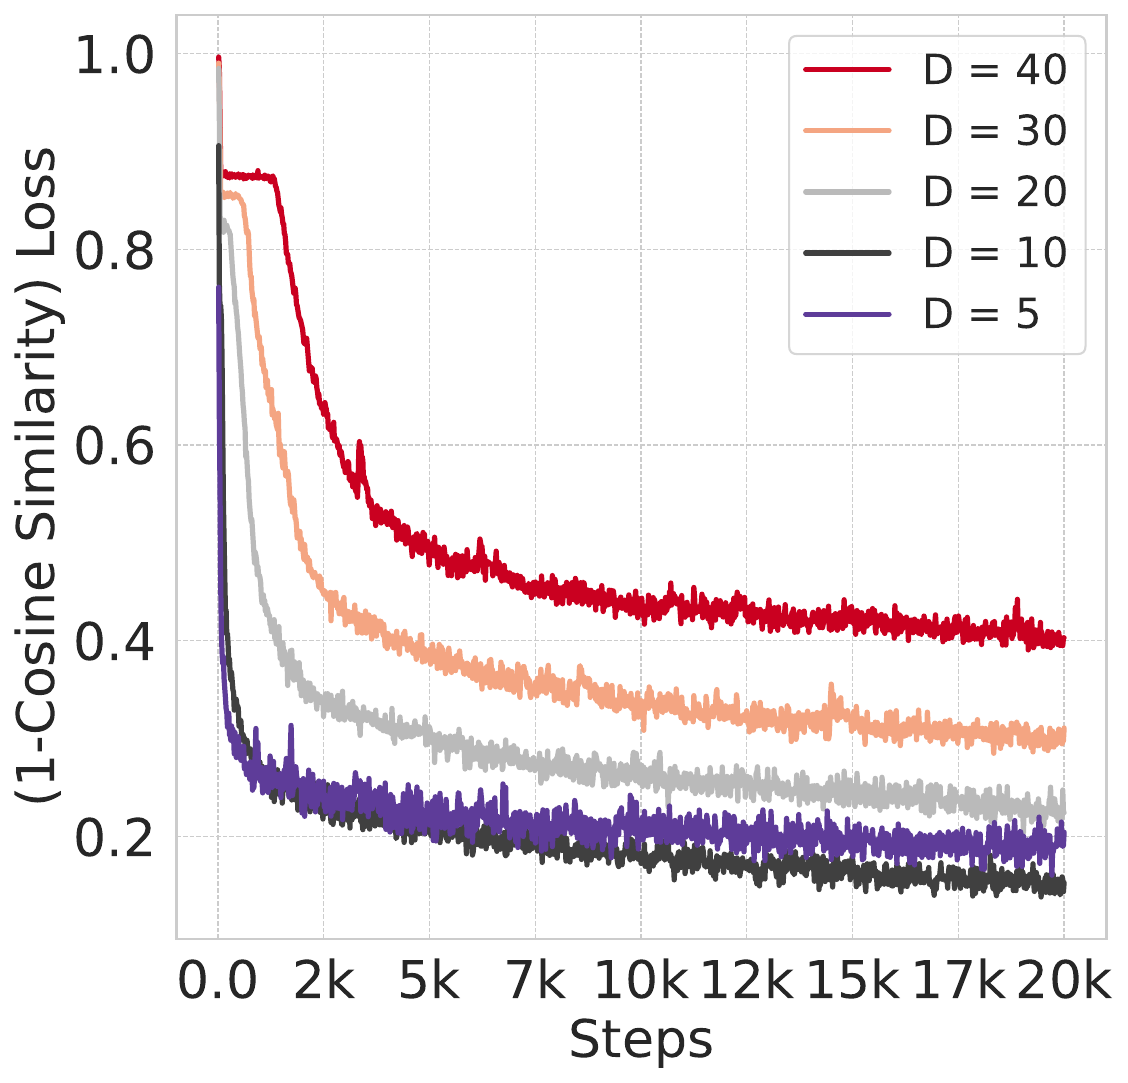}
    \endminipage\vspace{1em}
    \minipage{0.45\textwidth}
        \includegraphics[width=\linewidth]{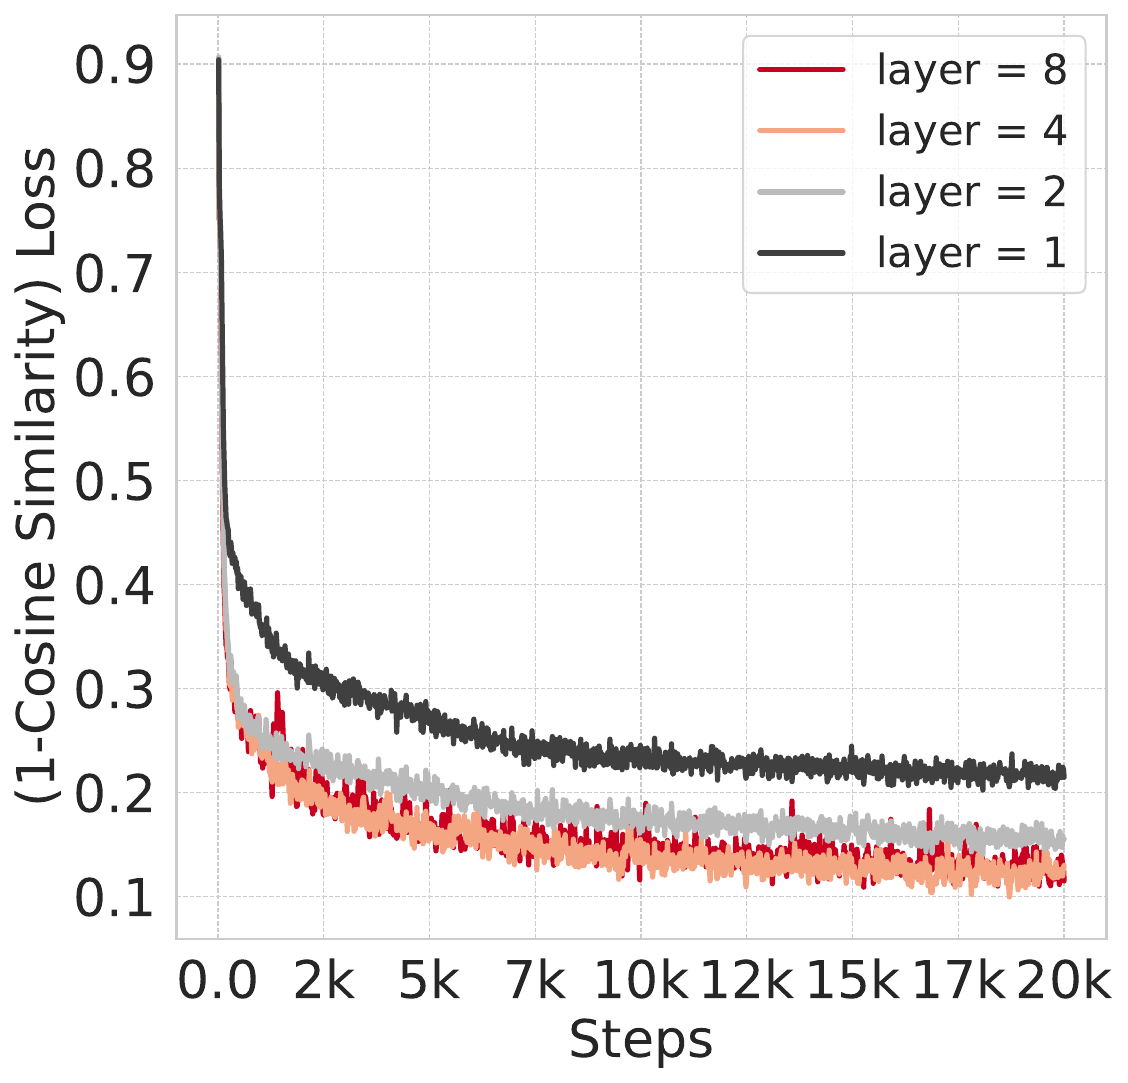}
    \endminipage\hfill
    \minipage{0.45\textwidth}
        \includegraphics[width=\linewidth]{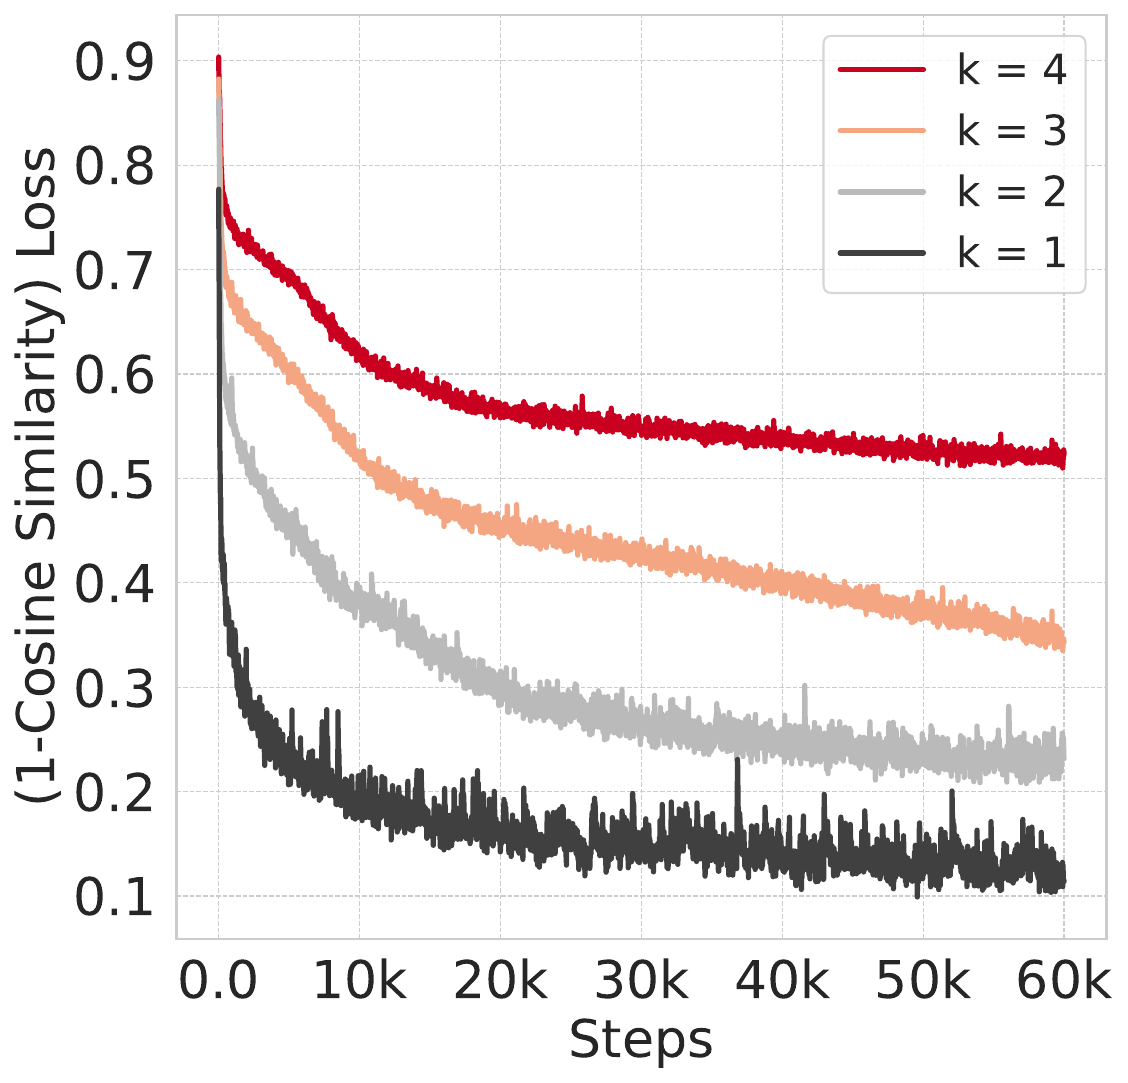}
    \endminipage
    \caption{\textbf{Convergence Results on Eigenvalue, Eigenvector Prediction with Different Parameters.}
    \emph{(1) Top left: Loss curve on eigenvalue prediction with different size of $D$}
    \emph{(2) Top middle: Loss curve on eigenvalue prediction with different number of layers}
    \emph{(3) Top right: Loss curve on eigenvector prediction with different size of $D$}
    \emph{(4) Bottom left: Top right: Loss curve on eigenvector prediction with different number of layers}
    \emph{(5) Bottom left: Loss curve on eigenvector prediction with different number of $k_{\text{train}}$}
    For (1), we observe that smaller $D$ is easier for transformers as they present lower losses.
    For (2), we see that with more layers, transformers are also capable of predicting eigenvalues more accurately.
    For (3), transformers also predict eigenvectors better when $D$ is small.
    For (4), similar to (2), transformers with more layers show improved performance.
    For (5), we want to highlight that the loss value is mainly affected by the fact that predicting 3rd or 4th eigenvectors is significantly harder, which contributes to a higher loss value.
    }
    \label{fig:loss}
\end{figure}

% \begin{figure}[!h]
% % \vspace{-1em}
% \minipage{0.5\textwidth}
% \minipage{0.5\textwidth}
% \includegraphics[width=\linewidth]{charts/relu_softmax_loss_d_5_plot.pdf}
% \endminipage\hfill
% \minipage{0.5\textwidth}
% \includegraphics[width=\textwidth]{charts/relu_softmax_loss_d_10_plot.pdf}
% \endminipage
% \endminipage\hfill
% \end{figure}

\begin{figure}[!h]
    \centering
    \begin{minipage}{0.45\textwidth}
        \centering
        \includegraphics[width=\linewidth]{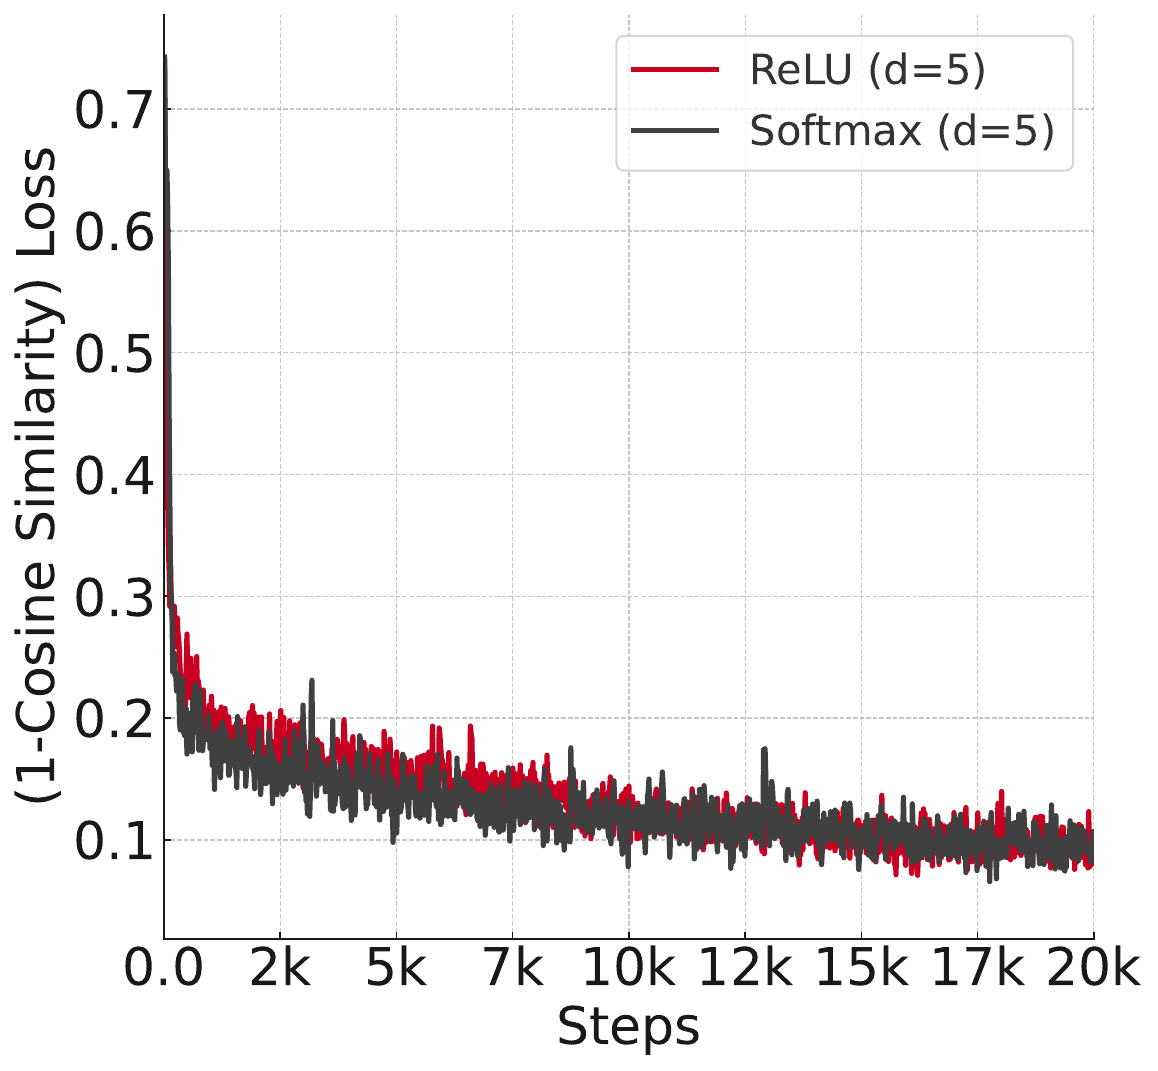}
    \end{minipage}
    \hfill % Adds space between the two minipages
    \begin{minipage}{0.45\textwidth}
        \centering
        \includegraphics[width=\linewidth]{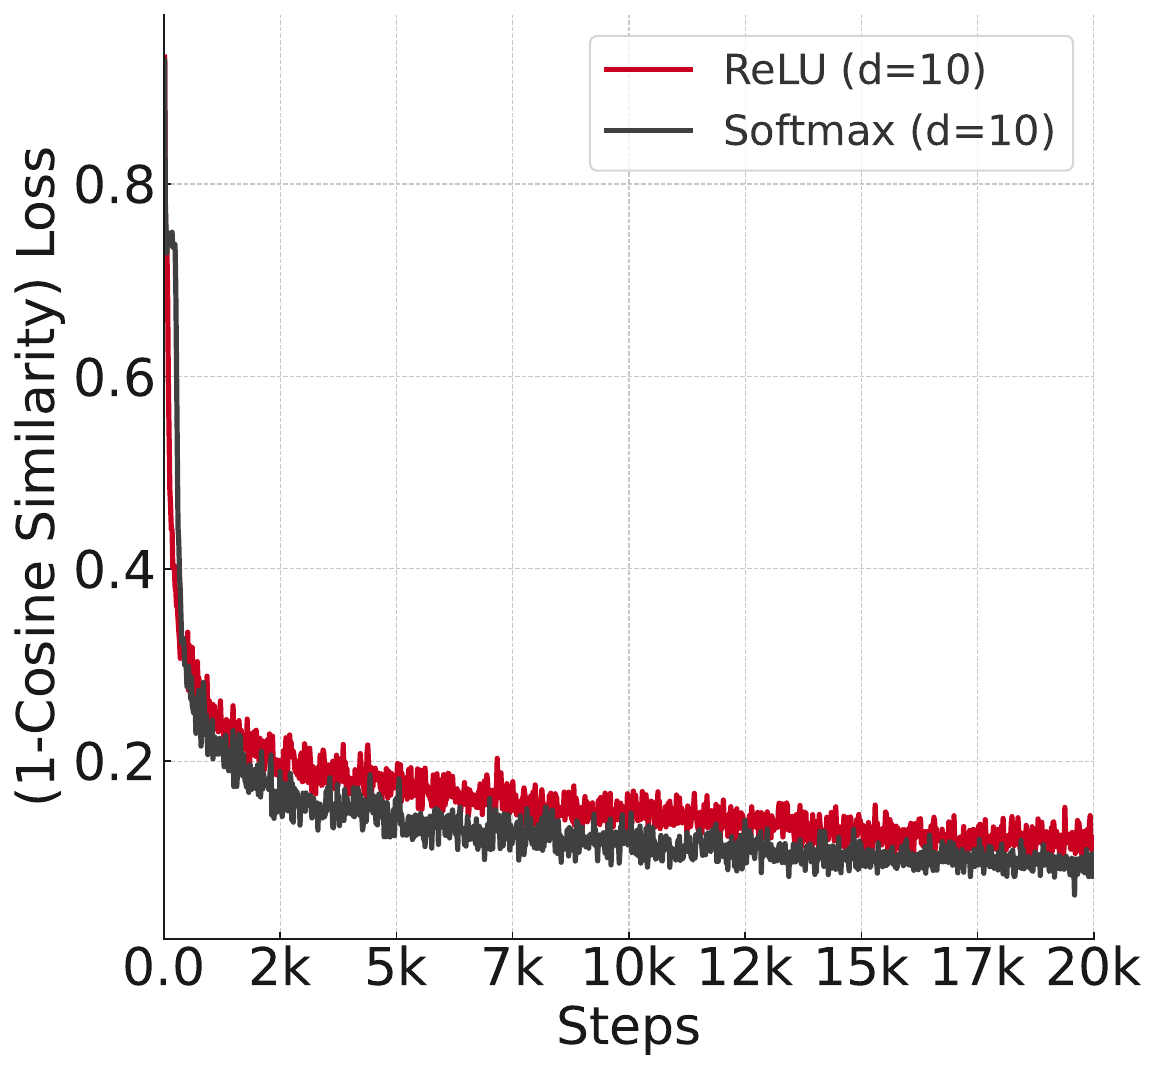}
    \end{minipage}
    \caption{\textbf{Loss Curve Comparison between Softmax and ReLU Transformers (Top-1 Eigenvector Prediction).}
    \emph{Left: $D=5$ }\emph{Right: $D=10$}
    We use a 3-layer, 2-head, 64 hidden dimension transformer to predict the top-1 eigenvector across all experiments in this figure. An explanation for the superior performance of ReLU transformers is that the normalizing behavior of Softmax can potentially hinder the PCA process.
    }
    \label{fig:relu_softmax1}
\end{figure}

\begin{figure}[!h]
    \centering
    \begin{minipage}{0.45\textwidth}
        \centering
        \includegraphics[width=\linewidth]{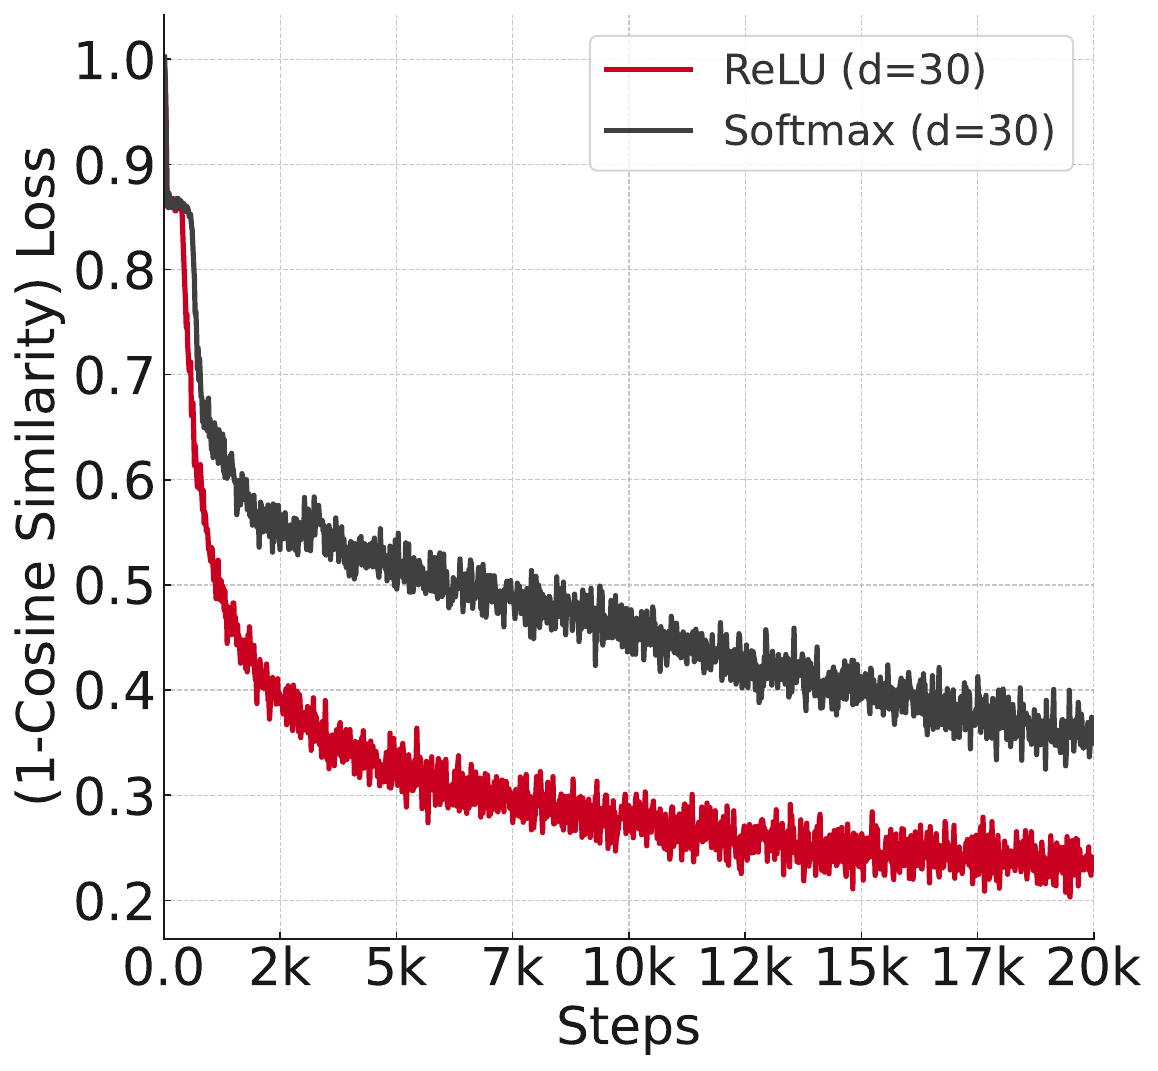}
    \end{minipage}
    \hfill % Adds space between the two minipages
    \begin{minipage}{0.45\textwidth}
        \centering
        \includegraphics[width=\linewidth]{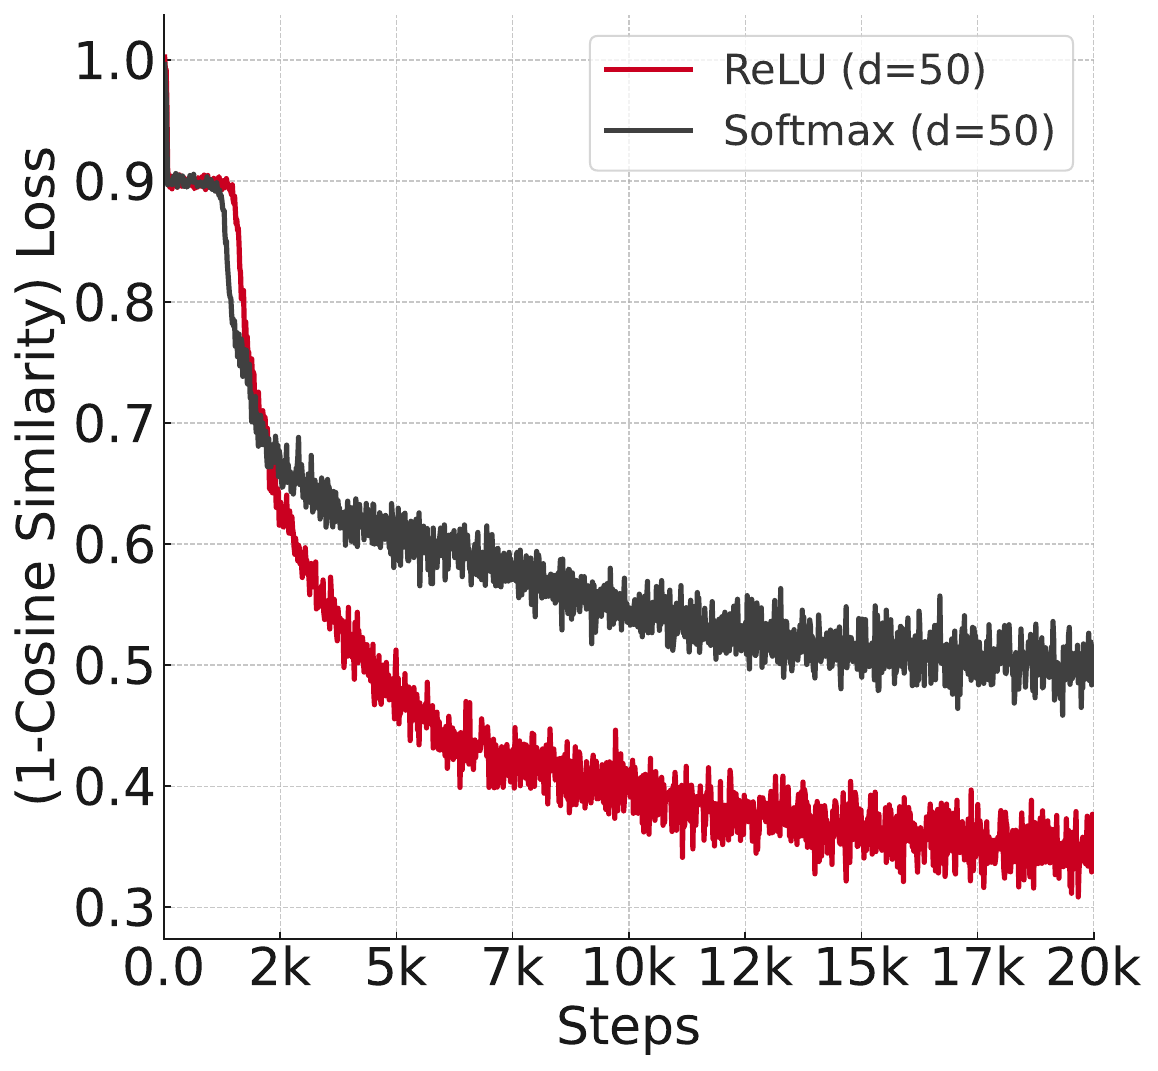}
    \end{minipage}
    
    \caption{\textbf{Loss Curve Comparison between Softmax and ReLU Transformers (Top-1 Eigenvector Prediction).}
    \emph{Left: $D=30$ }\emph{Right: $D=50$}
    We use a 3-layer, 2-head, 64 hidden dimension transformer to predict the top-1 eigenvector across all experiments in this figure. We also observe that the performance gap enlarges as $D$ increases, likely because the difference between eigenvectors becomes larger with increasing $D$, making the normalizing nature of Softmax unsuitable for PCA.
    }
    \label{fig:relu_softmax2}
\end{figure}

% \subsubsection{}
